# Supplementary material for: Extracting Einstein from the Loop-Level Double-Copy
Source: arXiv:2108.06798 ancillary file (2021-08-15)
Supplement: Supplementary file 1 [file guideToPDCfiles.pdf]

# Guide to Projective Double Copy Files

John Joseph M. Carrasco (carrasco@northwestern.edu)

Ingrid Vazquez-Holm (ingrid.vazquez.holm@gmail.com)

```
In[1]:= SetDirectory[NotebookDirectory[]];
```

```
In[2]:= FileNames["*"]
```

```
Out[2]= {guideToPDCfiles.nb, loop4pgravity.m, loop5pgravity.m, treesgravity.m}
```

This notebook shows how to use the gravity-theory numerator dressings in “treesgravity.m”, “loop4pgravity.m”, “loop5pgravity.m”.

We provide some helper functions in this notebook that automatically find e.g. which graphs are relevant to which cuts etc, largely based off of ideas described in <https://inspirehep.net/literature/1374212> .

---

## Some helpful definitions

### ulp

This is a shorthand for a Lorentz dot product. We call it ulp (unevaluated Lorentz product) because we are keeping it formal, without getting married to a metric or number of dimensions.

```
In[3]:= Attributes[ulp] = {Orderless}
ulp[- (a_), b_] := -ulp[a, b]
ulp[a_, (b_) + (c_)] := ulp[a, b] + ulp[a, c]
ulp[c_, (b_) * (a_)?NumberQ] := a * ulp[b, c]
Protect[ulp]
```

```
Out[3]= {Orderless}
```

```
Out[7]= {ulp}
```

### graphPlot

Our graphs are stored in vertex or node-oriented form. Mathematica likes to plot things in edge-oriented form so we need to be able to convert if we want to visualize. We include some mild intelligence for plotting massive legs in a different color than massless legs.

```

In[8]:= graphPlot[graph_, options___] :=
Module[{edges = First[toEdgeForm[graph]], massiveEdges},
  massiveEdges = Last /@ Normal@GroupBy[Select[edges,
    Head[#[[2]] /. -a_ -> a] === massive && #[[2, 2]] != 0 &], (# /. -a_ -> a) [[2, 2]] &];
  If[massiveEdges != {}, HighlightGraph[Graph[
    edges /. edge[a_ -> b_, c_] -> Labeled[DirectedEdge[a, b],
      c /. massive[aa_, bb_] -> DisplayForm[RowBox[{SuperscriptBox[aa, bb]}]]],
    GraphLayout -> "SpringElectricalEmbedding",
    PlotTheme -> "Classic", options], massiveEdges /.
    edge[a_ -> b_, c_] -> DirectedEdge[a, b]],
    Graph[edges /. edge[a_ -> b_, c_] -> Labeled[DirectedEdge[a, b],
      c /. massive[aa_, bb_] -> DisplayForm[RowBox[{SuperscriptBox[aa, bb]}]]],
    GraphLayout -> "SpringElectricalEmbedding",
    PlotTheme -> "Classic", EdgeStyle -> Directive[Gray, Opacity[1]], options]]]

```

```

In[9]:= toEdgeForm[nodeGraph[mynodes_]] :=
Module[{nodes = mynodes /. node[a___] -> node[{a]}},
  edgeFormGraph@Sort[
    Module[{whoITalkTo},
      Flatten[{
        Table[(
          If[Head[#1] != Times (* positive edge
            label *) && (whoITalkTo = Position[nodes, -#1]) != {},
            edgeFrom[
              neckl1,
              nodes[[whoITalkTo[[1, 1]]],
              #1], {}]) &] /@ neckl1[[1]],
          {neckl1, nodes}],
        Table[
          edgeFrom[nodes[[Position[nodes, edge] [[1, 1]]], node[{-edge}], edge],
          {edge, getNonConnectingEdges[nodes]}]
        ] /. edgeFrom[a_, b_, c_] -> edge[a -> b, c]],
    OrderedQ[Last /@ {#2, #1}] &] /. a_[ms[b_, c_]] -> massive[a[b], c]]

```

```

In[10]:= getNonConnectingEdges[list_] :=
First /@ Select[Tally[Flatten[list /. node[a___] -> a],
  ((SameQ@@ ({#1, #2} /. -a_ -> a)) &)], Last[#1] === 1 &]

```

```

In[11]:= graphPlot[ nodeGraph[{node[-e[ms[internal[1], m1]], k[ms[2, m1]], l[1]],
  node[k[ms[5, m2]], -l[2], e[ms[internal[8], m2]]], node[l[2], k[ms[1, m1]],
  e[ms[internal[1], m1]]], node[-l[1], k[ms[4, m2]], e[ms[internal[5], m2]]],
  node[-e[ms[internal[5], m2]], -e[ms[internal[8], m2]], k[3]]}] ]

```

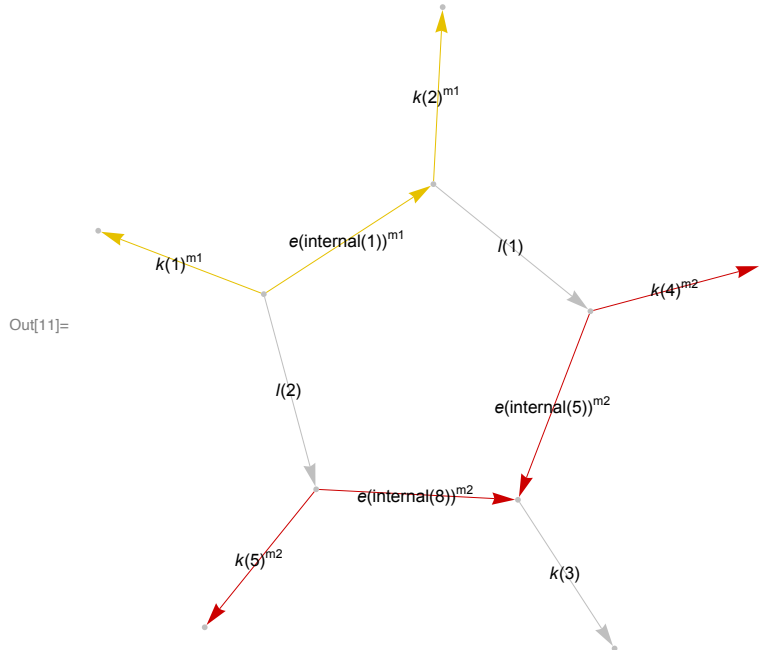

## gravSewing

Sewing gravitons D-dimensionally involves projecting out non-physical states.

```

In[12]:= gravSewing[expr_, bE_] :=
  Module[{myPols = Select[expr ~ extractType ~ ε, Head[#[[1]]] === Times &],
    curExpr = expr // Expand, newExpr, mypos, myneg},
    (* We find it somewhat more efficient to organize to sew one
      leg at a time. Scalar sewing is simply the product,
      but for graviton polarizations factorized into gluon polarizations
      we must sum over physical graviton states. *)
    Do[
      mypos = pols /. -a_ -> a;
      myneg = pols; Print["Sewing ..."]; Print[mypos]; Print[myneg];
      curExpr = FixedPoint[gravSewingPol[Collect[# // Expand, Power[ulp[_], mypos], _]
        Power[ulp[_], myneg], _], bE, mypos, myneg] &, {pols, myPols}];
    curExpr]

```

```

In[13]:= gravSewingPol[expr_, bE_, myPos_, myNeg_] := Module[{p = myPos[[1]]},
  expr /. {ulp[a_, myNeg]^2 × ulp[b_, myPos]^2 ⇒ proj[a, b, p],
    ulp[μ_, myNeg] × ulp[ν_, myNeg] ×
      ulp[ρ_, myPos] × ulp[σ_, myPos] ⇒ proj[μ, ν, ρ, σ, p],
    ulp[μ_, myNeg] × ulp[ν_, myNeg] × ulp[ρ_, myPos]^2 ⇒ proj[μ, ν, ρ, ρ, p],
    ulp[μ_, myNeg]^2 × ulp[ρ_, myPos] × ulp[σ_, myPos] ⇒ proj[μ, μ, ρ, σ, p],
    ulp[myNeg, myPos] × ulp[a_, myPos] × ulp[b_, myNeg] ⇒
      α1  $\left(\frac{1}{2} \times (1 + dd - 2) - \frac{1}{dd - 2}\right) * \text{proj}[a, b, p]$ ,
    ulp[myNeg, myPos]^2 ⇒ α2  $\left(\frac{1}{2} (dd - 2 + (dd - 2)^2) - 1\right) \}$  /.
  {proj[a_, b_, p_] ⇒ (pp[a, b, p]^2 - (pp[a, a, p] × pp[b, b, p]) / (-2 + dd)),
    proj[μ_, ν_, ρ_, σ_, p_] ⇒
      (1 / 2 (pp[μ, ρ, p] × pp[ν, σ, p] + pp[μ, σ, p] × pp[ν, ρ, p]) -
        (pp[μ, ν, p] × pp[ρ, σ, p]) / (-2 + dd))} /. pp[a_, b_, p_] ⇒ ulp[a, b] -
    (ulp[a, q] × ulp[b, p] + ulp[p, a] × ulp[b, q]) / ulp[p, q] // Expand]

```

additional Graph Tools relevant to graph isomorphism, generating graphs contributing to cuts, etc.

## Using the tree dressings

```

In[38]:= << "treesgravity.m"

```

We'll demonstrate how to use the files by performing some simple tasks.

Let's verify a graviton cut of the 4-point massless graviton amplitude:

This is the s-channel cut:

```

In[39]:= thisCut = {Atree[{k[1], k[2], l[1]}], Atree[{-l[1], k[3], k[4]}]};
thisCutMassRules = {}; (* No massive particles in 4-graviton scattering *)

```

We'll need some conservation of momentum rules

```

In[41]:= masslessLegs =
  Select[Flatten[thisCut /. Atree[a_] ⇒ a /. -a_ ⇒ a] /. thisCutMassRules // Union,
    Head[#] != massive &];

```

```

In[42]:= thisCutPols = ε /@masslessLegs;

```

```
In[43]:= theseCutRules =
  getIndepRules[thisCut /. thisCutMassRules, (thisCutMassRules /. Rule[b_, c_] =>
    (ulp[c, c] == (ulp[c, c] /. massive[i_, j_] => j /. ulp[0, 0] => 0)) // Flatten) ~
    Join~Map[ulp[#, #] == 0 &, masslessLegs]];
thesePolRules = getPolRules[thisCut /. thisCutMassRules, thisCutPols];
backToBasis[expr_] := expr //. theseCutRules //. thesePolRules;
```

Conservation of momentum rules:

```
In[46]:= theseCutRules
Out[46]:= {ulp[l[1], l[1]] -> 0, ulp[k[4], l[1]] -> 0, ulp[k[4], k[4]] -> 0,
  ulp[k[3], l[1]] -> 0, ulp[k[3], k[4]] -> 0, ulp[k[3], k[3]] -> 0,
  ulp[k[2], l[1]] -> 0, ulp[k[2], k[3]] -> -ulp[k[2], k[4]],
  ulp[k[2], k[2]] -> 0, ulp[k[1], l[1]] -> 0, ulp[k[1], k[4]] -> -ulp[k[2], k[4]],
  ulp[k[1], k[3]] -> ulp[k[2], k[4]], ulp[k[1], k[2]] -> 0, ulp[k[1], k[1]] -> 0}
```

Polarization rules (recall graviton polarizations factorize into products of gluon polarizations):

```
In[47]:= thesePolRules
Out[47]:= {ulp[ε[-k[1]], ε[-k[1]]] -> 0, ulp[ε[k[1]], ε[k[1]]] -> 0,
  ulp[ε[-k[2]], ε[-k[2]]] -> 0, ulp[ε[k[2]], ε[k[2]]] -> 0,
  ulp[ε[-k[3]], ε[-k[3]]] -> 0, ulp[ε[k[3]], ε[k[3]]] -> 0, ulp[ε[-k[4]], ε[-k[4]]] -> 0,
  ulp[ε[k[4]], ε[k[4]]] -> 0, ulp[ε[-l[1]], ε[-l[1]]] -> 0, ulp[ε[l[1]], ε[l[1]]] -> 0,
  ulp[k[3], ε[-k[1]]] -> -ulp[k[4], ε[-k[1]]] + ulp[l[1], ε[-k[1]]],
  ulp[k[2], ε[-k[1]]] -> -ulp[l[1], ε[-k[1]]], ulp[k[1], ε[-k[1]]] -> 0,
  ulp[k[3], ε[k[1]]] -> -ulp[k[4], ε[k[1]]] + ulp[l[1], ε[k[1]]],
  ulp[k[2], ε[k[1]]] -> -ulp[l[1], ε[k[1]]], ulp[k[1], ε[k[1]]] -> 0,
  ulp[k[3], ε[-k[2]]] -> -ulp[k[4], ε[-k[2]]] + ulp[l[1], ε[-k[2]]],
  ulp[k[2], ε[-k[2]]] -> 0, ulp[k[1], ε[-k[2]]] -> -ulp[l[1], ε[-k[2]]],
  ulp[k[3], ε[k[2]]] -> -ulp[k[4], ε[k[2]]] + ulp[l[1], ε[k[2]]],
  ulp[k[2], ε[k[2]]] -> 0, ulp[k[1], ε[k[2]]] -> -ulp[l[1], ε[k[2]]],
  ulp[k[4], ε[-k[3]]] -> ulp[l[1], ε[-k[3]]], ulp[k[3], ε[-k[3]]] -> 0,
  ulp[k[1], ε[-k[3]]] -> -ulp[k[2], ε[-k[3]]] - ulp[l[1], ε[-k[3]]],
  ulp[k[4], ε[k[3]]] -> ulp[l[1], ε[k[3]]], ulp[k[3], ε[k[3]]] -> 0,
  ulp[k[1], ε[k[3]]] -> -ulp[k[2], ε[k[3]]] - ulp[l[1], ε[k[3]]],
  ulp[k[4], ε[-k[4]]] -> 0, ulp[k[3], ε[-k[4]]] -> ulp[l[1], ε[-k[4]]],
  ulp[k[1], ε[-k[4]]] -> -ulp[k[2], ε[-k[4]]] - ulp[l[1], ε[-k[4]]],
  ulp[k[4], ε[k[4]]] -> 0, ulp[k[3], ε[k[4]]] -> ulp[l[1], ε[k[4]]],
  ulp[k[1], ε[k[4]]] -> -ulp[k[2], ε[k[4]]] - ulp[l[1], ε[k[4]]],
  ulp[l[1], ε[-l[1]]] -> 0, ulp[k[3], ε[-l[1]]] -> -ulp[k[4], ε[-l[1]]],
  ulp[k[1], ε[-l[1]]] -> -ulp[k[2], ε[-l[1]]], ulp[l[1], ε[l[1]]] -> 0,
  ulp[k[3], ε[l[1]]] -> -ulp[k[4], ε[l[1]]], ulp[k[1], ε[l[1]]] -> -ulp[k[2], ε[l[1]]]}
```

Individual graphs contributing to the cut.

```
In[48]:= theseGraphs = unOrderedGraphs[#{#}, thisCutMassRules] & /@ thisCut;
```

Here are the graphs contributing on every side of the cut -- in this case, three-point graphs.

```
In[49]:= theseGraphs
```

```
Out[49]= {{nodeGraph[{node[k[1], k[2], l[1]]}], {nodeGraph[{node[-l[1], k[3], k[4]]}]}}
```

```
In[50]:= graphPlot /@ Flatten@theseGraphs
```

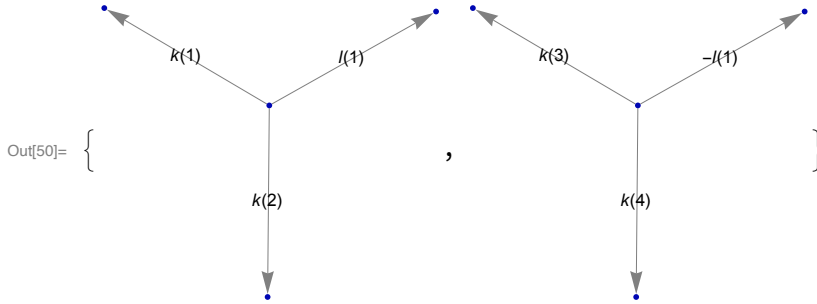

We'll dress these graphs with their amplitudes, then we'll have to preform the state sum over the gravitons.

```
In[51]:= cutDressings =
```

```
(Times @@ Table[Total[(getCutContribution[#1, treeGraph /@ allTreeGraphNames,
gravityNumerator] &) /@ dat],
{dat, theseGraphs}] /. theseCutRules /. thesePolRules) // Together;
```

```
In[52]:= nums = ExpandAll[Numerator[cutDressings]];
```

```
denoms = Denominator[cutDressings];
```

Sewing gravitons means summing over all valid graviton states:

```
In[54]:= sewnCut = FixedPoint[(gravSewing[#, backToBasis] // Expand) &, nums] / denoms;
```

Sewing ...

$$\varepsilon[l[1]]$$

$$\varepsilon[-l[1]]$$

That expression must match what we get when we dress the 4-point s-channel graph with the relevant dressing and apply cut conditions to the resulting expression:

```
In[55]:= sewnCut // FullSimplify
```

```
Out[55]= (-ulp[k[2], ε[k[4]]] × ulp[l[1], ε[k[3]]] × ulp[ε[k[1]], ε[k[2]]] +
ulp[k[2], ε[k[3]]] × ulp[l[1], ε[k[4]]] × ulp[ε[k[1]], ε[k[2]]] -
ulp[l[1], ε[k[2]]] × ulp[l[1], ε[k[4]]] × ulp[ε[k[1]], ε[k[3]]] +
ulp[l[1], ε[k[2]]] × ulp[l[1], ε[k[3]]] × ulp[ε[k[1]], ε[k[4]]] +
ulp[l[1], ε[k[1]]] × ulp[l[1], ε[k[4]]] × ulp[ε[k[2]], ε[k[3]]] -
ulp[l[1], ε[k[1]]] × ulp[l[1], ε[k[3]]] × ulp[ε[k[2]], ε[k[4]]] +
(ulp[k[4], ε[k[2]]] × ulp[l[1], ε[k[1]]] - ulp[k[4], ε[k[1]]] × ulp[l[1], ε[k[2]]] +
ulp[k[2], k[4]] × ulp[ε[k[1]], ε[k[2]]]) × ulp[ε[k[3]], ε[k[4]]])2
```

```
In[56]:= dressedCut =
  getCutContribution[#, treeGraph /@ allTreeGraphNames, gravityNumerator] & /@
  unOrderedGraphs[thisCut, thisCutMassRules] // Total // backToBasis // Simplify

Out[56]= (-ulp[k[2], ε[k[4]]] × ulp[l[1], ε[k[3]]] × ulp[ε[k[1]], ε[k[2]]] +
  ulp[k[2], ε[k[3]]] × ulp[l[1], ε[k[4]]] × ulp[ε[k[1]], ε[k[2]]] -
  ulp[l[1], ε[k[2]]] × ulp[l[1], ε[k[4]]] × ulp[ε[k[1]], ε[k[3]]] +
  ulp[l[1], ε[k[2]]] × ulp[l[1], ε[k[3]]] × ulp[ε[k[1]], ε[k[4]]] +
  ulp[l[1], ε[k[1]]] × ulp[l[1], ε[k[4]]] × ulp[ε[k[2]], ε[k[3]]] -
  ulp[l[1], ε[k[1]]] × ulp[l[1], ε[k[3]]] × ulp[ε[k[2]], ε[k[4]]] +
  ulp[k[4], ε[k[2]]] × ulp[l[1], ε[k[1]]] × ulp[ε[k[3]], ε[k[4]]] -
  ulp[k[4], ε[k[1]]] × ulp[l[1], ε[k[2]]] × ulp[ε[k[3]], ε[k[4]]] +
  ulp[k[2], k[4]] × ulp[ε[k[1]], ε[k[2]]] × ulp[ε[k[3]], ε[k[4]]])2
```

This cut is satisfied if the difference between those expressions vanishes:

```
In[57]:= (sewnCut - dressedCut // Expand) === 0

Out[57]= True
```

## Let's build the 5-point 3-graviton 2-scalar tree-amplitude from graphs

```
In[58]:= allTreeGraphNames

Out[58]= {{3, hhh}, {3, hss}, {4, hhhh}, {4, hhss, 12, 34}, {4, hhss, 41, 23},
  {4, ssss, 12, 34}, {5, hssss, 12, 3, 45}, {5, hssss, 45, 1, 23},
  {5, hhhss, 23, 1, 45}, {5, hhhss, 51, 4, 23}, {5, hhhss, 34, 2, 51}}

In[59]:= fivePointAmplitudeTreeDesc = {Atree[k /@ Range[5]]}

Out[59]= {Atree[{k[1], k[2], k[3], k[4], k[5]}]}

In[60]:= thisCut = fivePointAmplitudeTreeDesc;
  thisCutMassRules = {k[4] → massive[k[4], m[1]], k[5] → massive[k[5], m[1]]};

We're making legs 4 and 5 massive scalars.

We'll need some conservation of momentum rules

In[61]:= masslessLegs =
  Select[Flatten[fivePointAmplitudeTreeDesc /. Atree[a__] → a /. -a_ → a] /.
    thisCutMassRules // Union,
    Head[#] != massive &];

In[62]:= thisCutPolS = ε /@ masslessLegs;
```

```
In[63]:= theseCutRules =
  getIndepRules[thisCut /. thisCutMassRules, (thisCutMassRules /. Rule[b_, c_] =>
    (ulp[c, c] == (ulp[c, c] /. massive[i_, j_] => j /. ulp[0, 0] => 0)) // Flatten) ~
    Join~Map[ulp[#, #] == 0 &, masslessLegs]];
thesePolRules = getPolRules[thisCut /. thisCutMassRules, thisCutPols];
backToBasis[expr_] := expr /. theseCutRules /. thesePolRules;
```

Conservation of momentum rules:

```
In[66]:= theseCutRules
Out[66]:= {ulp[k[ms[4, m[1]]], k[ms[4, m[1]]]] -> ulp[k[ms[5, m[1]]], k[ms[5, m[1]]]],
  ulp[m[1], m[1]] -> ulp[k[ms[5, m[1]]], k[ms[5, m[1]]]],
  ulp[k[3], k[3]] -> 0, ulp[k[2], k[3]] ->
    -ulp[k[2], k[ms[4, m[1]]]] - ulp[k[2], k[ms[5, m[1]]]] - ulp[k[3], k[ms[4, m[1]]]] -
    ulp[k[3], k[ms[5, m[1]]]] - ulp[k[ms[4, m[1]]], k[ms[5, m[1]]]] -
    ulp[k[ms[5, m[1]]], k[ms[5, m[1]]]], ulp[k[2], k[2]] -> 0,
  ulp[k[1], k[ms[5, m[1]]]] -> -ulp[k[2], k[ms[5, m[1]]]] - ulp[k[3], k[ms[5, m[1]]]] -
    ulp[k[ms[4, m[1]]], k[ms[5, m[1]]]] - ulp[k[ms[5, m[1]]], k[ms[5, m[1]]]],
  ulp[k[1], k[ms[4, m[1]]]] -> -ulp[k[2], k[ms[4, m[1]]]] - ulp[k[3], k[ms[4, m[1]]]] -
    ulp[k[ms[4, m[1]]], k[ms[5, m[1]]]] - ulp[k[ms[5, m[1]]], k[ms[5, m[1]]]],
  ulp[k[1], k[3]] -> ulp[k[2], k[ms[4, m[1]]]] + ulp[k[2], k[ms[5, m[1]]]] +
    ulp[k[ms[4, m[1]]], k[ms[5, m[1]]]] + ulp[k[ms[5, m[1]]], k[ms[5, m[1]]]],
  ulp[k[1], k[2]] -> ulp[k[3], k[ms[4, m[1]]]] + ulp[k[3], k[ms[5, m[1]]]] +
    ulp[k[ms[4, m[1]]], k[ms[5, m[1]]]] +
    ulp[k[ms[5, m[1]]], k[ms[5, m[1]]]], ulp[k[1], k[1]] -> 0}
```

Polarization rules (recall graviton polarizations factorize into products of gluon polarizations):

```
In[67]:= thesePolRules
Out[67]:= {ulp[ε[-k[1]], ε[-k[1]]] -> 0, ulp[ε[k[1]], ε[k[1]]] -> 0, ulp[ε[-k[2]], ε[-k[2]]] -> 0,
  ulp[ε[k[2]], ε[k[2]]] -> 0, ulp[ε[-k[3]], ε[-k[3]]] -> 0, ulp[ε[k[3]], ε[k[3]]] -> 0,
  ulp[k[2], ε[-k[1]]] -> -ulp[k[3], ε[-k[1]]] - ulp[k[ms[4, m[1]]], ε[-k[1]]] -
    ulp[k[ms[5, m[1]]], ε[-k[1]]], ulp[k[1], ε[-k[1]]] -> 0, ulp[k[2], ε[k[1]]] ->
    -ulp[k[3], ε[k[1]]] - ulp[k[ms[4, m[1]]], ε[k[1]]] - ulp[k[ms[5, m[1]]], ε[k[1]]],
  ulp[k[1], ε[k[1]]] -> 0, ulp[k[2], ε[-k[2]]] -> 0,
  ulp[k[1], ε[-k[2]]] -> -ulp[k[3], ε[-k[2]]] - ulp[k[ms[4, m[1]]], ε[-k[2]]] -
    ulp[k[ms[5, m[1]]], ε[-k[2]]], ulp[k[2], ε[k[2]]] -> 0, ulp[k[1], ε[k[2]]] ->
    -ulp[k[3], ε[k[2]]] - ulp[k[ms[4, m[1]]], ε[k[2]]] - ulp[k[ms[5, m[1]]], ε[k[2]]],
  ulp[k[3], ε[-k[3]]] -> 0, ulp[k[1], ε[-k[3]]] -> -ulp[k[2], ε[-k[3]]] -
    ulp[k[ms[4, m[1]]], ε[-k[3]]] - ulp[k[ms[5, m[1]]], ε[-k[3]]],
  ulp[k[3], ε[k[3]]] -> 0, ulp[k[1], ε[k[3]]] ->
    -ulp[k[2], ε[k[3]]] - ulp[k[ms[4, m[1]]], ε[k[3]]] - ulp[k[ms[5, m[1]]], ε[k[3]]]}
```

These graphs contribute to the amplitude:



In[68]:= `graphPlot /@ unOrderedGraphs[thisCut, thisCutMassRules]`

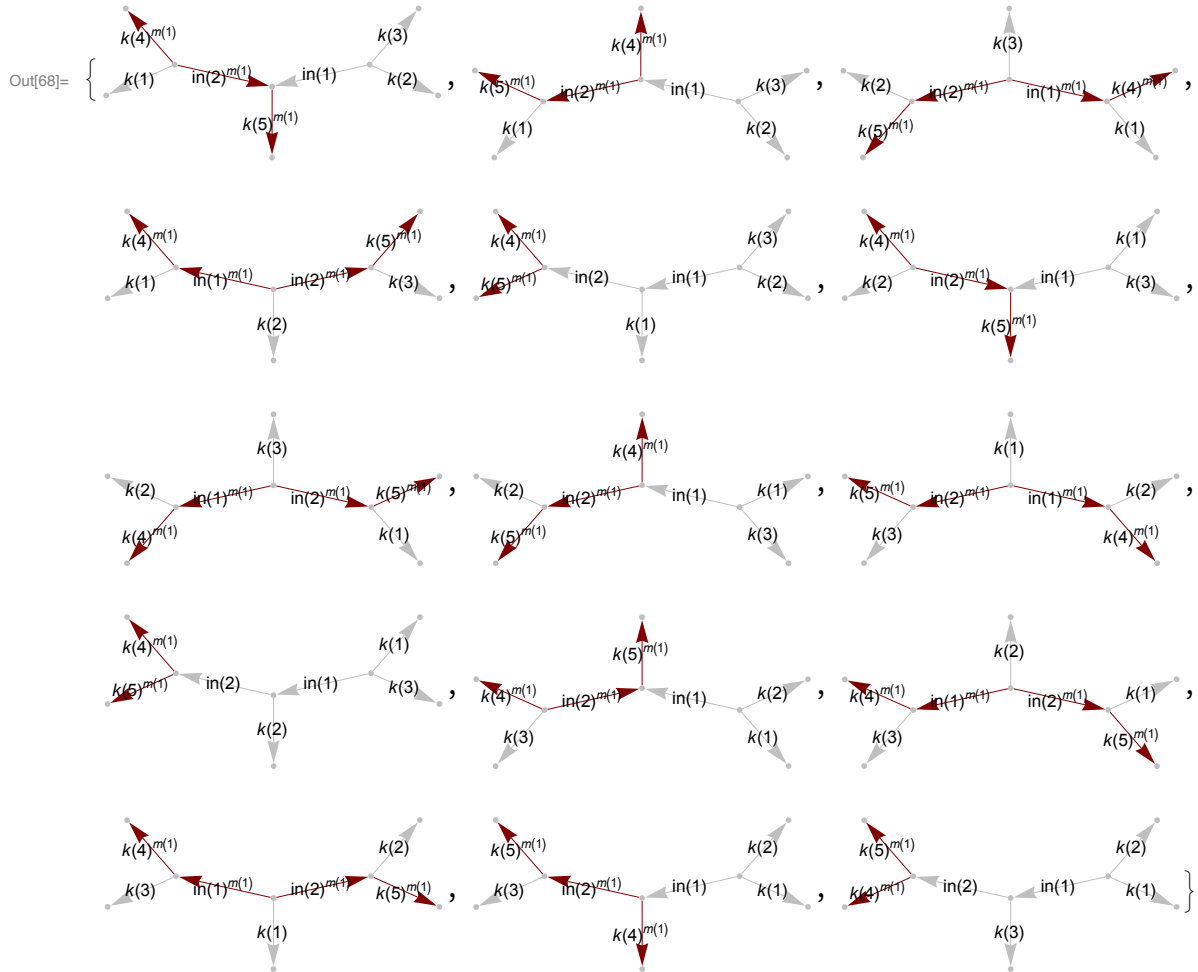

Which graphs were these? And how do we need to relabel from canonical definitions to apply to this amplitude?

In[69]:= `Table[`  
`{myGrName = First@Select[allTreeGraphNames, isIsomorphic[treeGraph[#, grph] &],`  
`(graphPlot@treeGraph@myGrName /. internal -> i) /. e[___] -> "",`  
`Select[isomorphicEdgeRule[treeGraph@myGrName, grph], Head[First[#]] === k &]},`  
`{grph, unOrderedGraphs[thisCut, thisCutMassRules]}`  
`]`

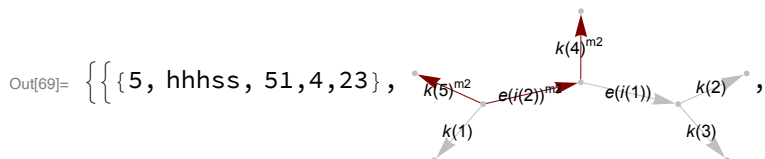

`{k[ms[5, m2]] -> k[ms[4, m[1]]], k[ms[4, m2]] -> k[ms[5, m[1]]]}`

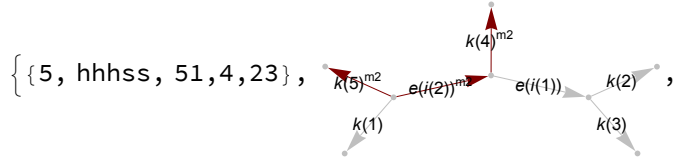

$$\{ k[\text{ms}[5, \text{m2}]] \rightarrow k[\text{ms}[5, \text{m}[1]]], k[\text{ms}[4, \text{m2}]] \rightarrow k[\text{ms}[4, \text{m}[1]]] \},$$

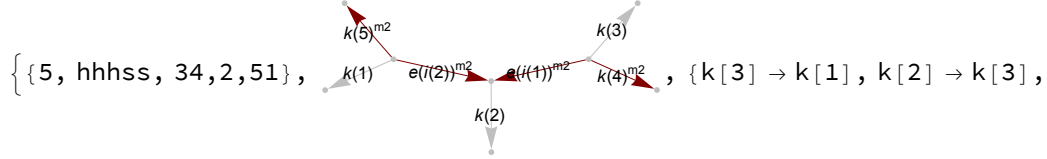

$$k[1] \rightarrow k[2], k[\text{ms}[5, \text{m2}]] \rightarrow k[\text{ms}[5, \text{m}[1]]], k[\text{ms}[4, \text{m2}]] \rightarrow k[\text{ms}[4, \text{m}[1]]] \},$$

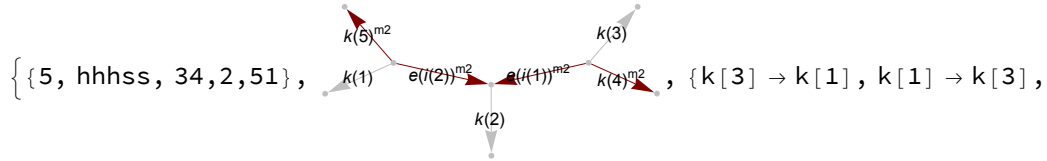

$$k[\text{ms}[5, \text{m2}]] \rightarrow k[\text{ms}[5, \text{m}[1]]], k[\text{ms}[4, \text{m2}]] \rightarrow k[\text{ms}[4, \text{m}[1]]] \},$$

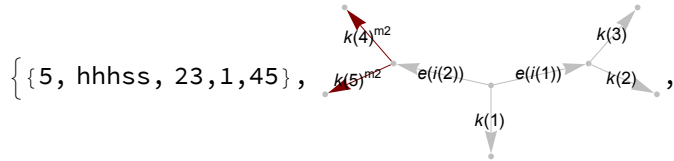

$$\{ k[\text{ms}[5, \text{m2}]] \rightarrow k[\text{ms}[5, \text{m}[1]]], k[\text{ms}[4, \text{m2}]] \rightarrow k[\text{ms}[4, \text{m}[1]]] \},$$

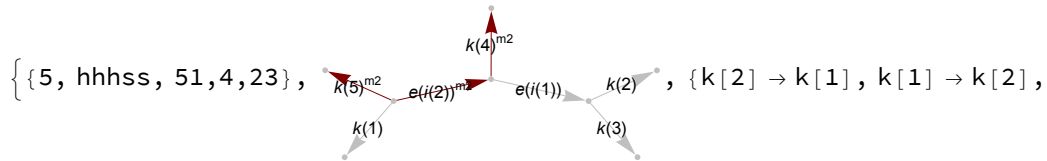

$$k[\text{ms}[5, \text{m2}]] \rightarrow k[\text{ms}[4, \text{m}[1]]], k[\text{ms}[4, \text{m2}]] \rightarrow k[\text{ms}[5, \text{m}[1]]] \},$$

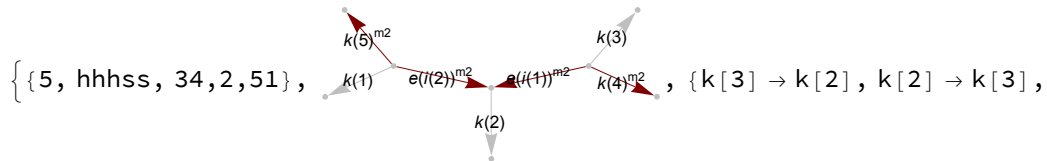

$$k[\text{ms}[5, \text{m2}]] \rightarrow k[\text{ms}[5, \text{m}[1]]], k[\text{ms}[4, \text{m2}]] \rightarrow k[\text{ms}[4, \text{m}[1]]] \},$$

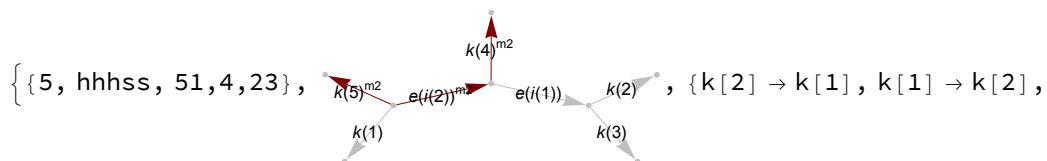

$$k[ms[5, m2]] \rightarrow k[ms[5, m[1]]], k[ms[4, m2]] \rightarrow k[ms[4, m[1]]], \}$$

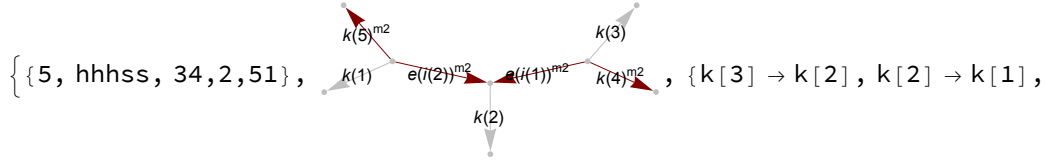

$$k[1] \rightarrow k[3], k[ms[5, m2]] \rightarrow k[ms[5, m[1]]], k[ms[4, m2]] \rightarrow k[ms[4, m[1]]], \}$$

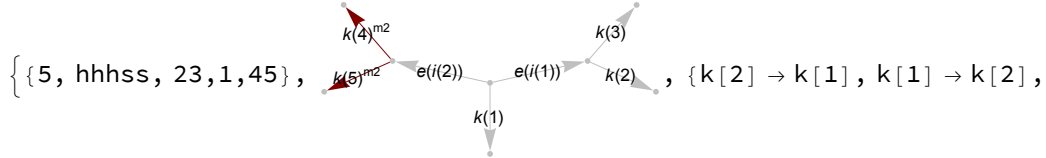

$$k[ms[5, m2]] \rightarrow k[ms[5, m[1]]], k[ms[4, m2]] \rightarrow k[ms[4, m[1]]], \}$$

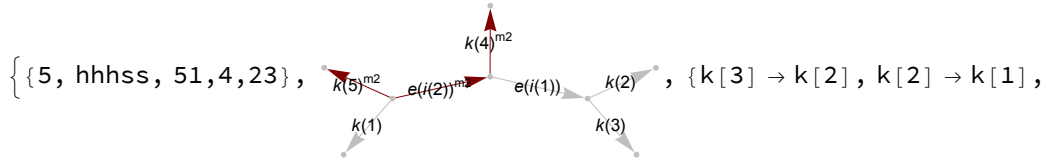

$$k[1] \rightarrow k[3], k[ms[5, m2]] \rightarrow k[ms[4, m[1]]], k[ms[4, m2]] \rightarrow k[ms[5, m[1]]], \}$$

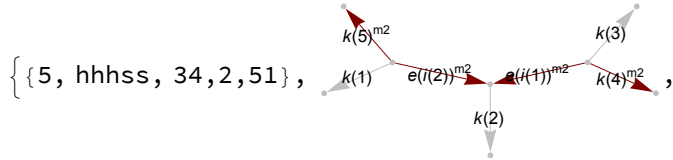

$$\{k[ms[5, m2]] \rightarrow k[ms[5, m[1]]], k[ms[4, m2]] \rightarrow k[ms[4, m[1]]], \}$$

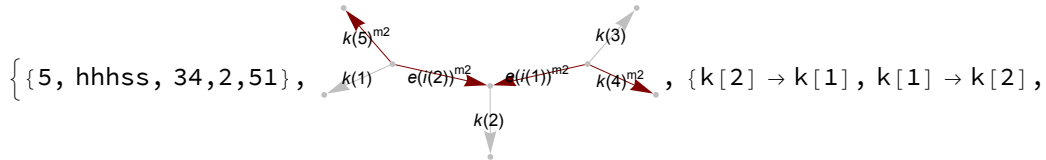

$$k[ms[5, m2]] \rightarrow k[ms[5, m[1]]], k[ms[4, m2]] \rightarrow k[ms[4, m[1]]], \}$$

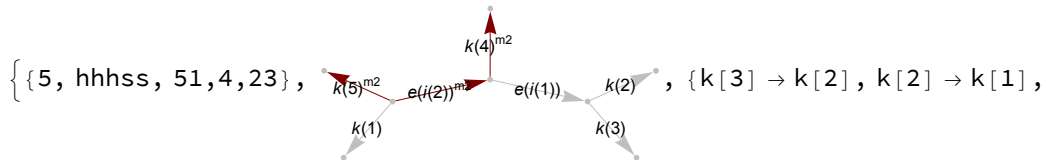

$$k[1] \rightarrow k[3], k[ms[5, m2]] \rightarrow k[ms[5, m[1]]], k[ms[4, m2]] \rightarrow k[ms[4, m[1]]], \}$$

$$\left\{ \{5, \text{hhhss}, 23, 1, 45\}, \{k[3] \rightarrow k[2], k[2] \rightarrow k[1], k[1] \rightarrow k[3], k[\text{ms}[5, m2]] \rightarrow k[\text{ms}[5, m[1]]], k[\text{ms}[4, m2]] \rightarrow k[\text{ms}[4, m[1]]]\} \right\}$$

The full five-point tree amplitude we scoop from the numerator dressings of the canonical graphs, appropriately relabeled:

```
In[70]:= fivePointAmplitude =
  getCutContribution[#, treeGraph /@ allTreeGraphNames, gravityNumerator] & /@
  unOrderedGraphs[thisCut, thisCutMassRules] // Total // backToBasis
```

Out[70]=

$$\frac{\left( \frac{((\dots 1 \dots) (\dots 1 \dots) \text{ulp}[\varepsilon[k[1]], \varepsilon[k[2]]] + \dots 15 \dots + \dots 1 \dots)^2}{2 (\dots 1 \dots) (2 \text{ulp}[k[\text{ms}[4, m[1]]], k[\text{ms}[5, m[1]]]] + 2 \text{ulp}[k[\text{ms}[5, m[1]]], k[\text{ms}[5, m[1]]]])} + \frac{(\dots 1 \dots)^2}{(\dots 1 \dots)} + \dots 11 \dots + \frac{(\dots 1 \dots)}{(\dots 1 \dots)} + \frac{(\dots 1 \dots + \dots 10 \dots + \dots 1 \dots)^2}{2 \text{ulp}[(\dots 1 \dots) (2 \text{ulp}[k[2], k[\text{ms}[5, \dots 1 \dots]]] + 2 (\dots 1 \dots + 2 (\dots 1 \dots)))} \right)$$

large output    [show less](#)    [show more](#)    [show all](#)    [set size limit...](#)

Does this satisfy gauge invariance? Sure. Since it's a little lengthy, it's quickest to see this when we plug in numbers. So let's find some prime numbers for the basis Lorentz invariants:

```
In[71]:= someRandomMomenta =
  Map[# -> RandomPrime[{10^3, 10^6}] &, fivePointAmplitude // extractType[#, ulp] &]
```

```
Out[71]:= {ulp[k[2], k[ms[4, m[1]]]] -> 67891, ulp[k[2], k[ms[5, m[1]]]] -> 17377,
  ulp[k[2], ε[k[3]]] -> 934793, ulp[k[3], k[ms[4, m[1]]]] -> 70381,
  ulp[k[3], k[ms[5, m[1]]]] -> 888857, ulp[k[3], ε[k[1]]] -> 107981,
  ulp[k[3], ε[k[2]]] -> 280681, ulp[k[ms[4, m[1]]], k[ms[5, m[1]]]] -> 260339,
  ulp[k[ms[4, m[1]]], ε[k[1]]] -> 690119, ulp[k[ms[4, m[1]]], ε[k[2]]] -> 555829,
  ulp[k[ms[4, m[1]]], ε[k[3]]] -> 373649, ulp[k[ms[5, m[1]]], k[ms[5, m[1]]]] -> 3169,
  ulp[k[ms[5, m[1]]], ε[k[1]]] -> 727981, ulp[k[ms[5, m[1]]], ε[k[2]]] -> 6701,
  ulp[k[ms[5, m[1]]], ε[k[3]]] -> 244091, ulp[ε[k[1]], ε[k[2]]] -> 767489,
  ulp[ε[k[1]], ε[k[3]]] -> 903607, ulp[ε[k[2]], ε[k[3]]] -> 674273}
```

With these kinematics the full amplitude is the following number:

```
In[72]:= fivePointAmplitude /. someRandomMomenta // Expand
```

```
Out[72]:= 1424778827527343953520976057800352405537951692049754685600180490465377488
  675 / 6069633798962622032776252285030317967531462644469632
```

We see that if we replace any of the graviton's polarizations with its associated momenta then the amplitude vanishes via the ward identity:

```

In[73]:= (fivePointAmplitude /.  $\varepsilon[k[1]] \rightarrow k[1]$  // backToBasis) /. someRandomMomenta // Expand
Out[73]= 0

In[74]:= (fivePointAmplitude /.  $\varepsilon[k[2]] \rightarrow k[2]$  // backToBasis) /. someRandomMomenta // Expand
Out[74]= 0

In[75]:= (fivePointAmplitude /.  $\varepsilon[k[3]] \rightarrow k[3]$  // backToBasis) /. someRandomMomenta // Expand
Out[75]= 0

```

## Using the one loop 4pt dressings

```

In[76]:= << "loop4pgravity.m";

In[77]:= graphPlot /@ (oneLoopGraph /@ oneLoop4pGraphNames /. internal  $\rightarrow$  i)

```

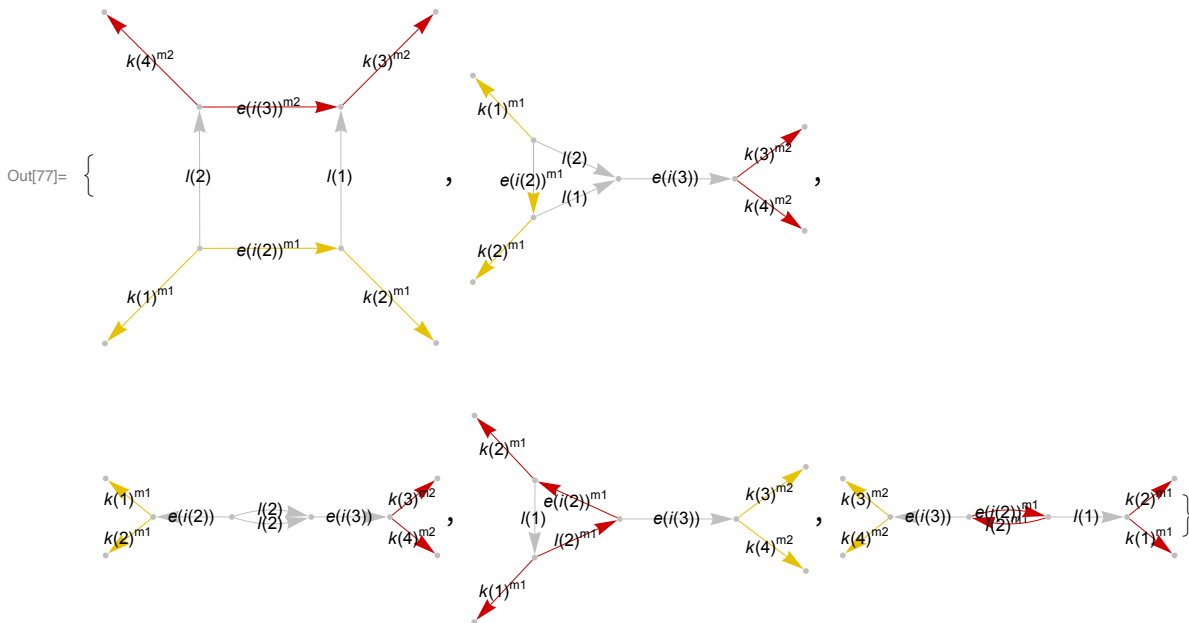

## Using the dressings to verify a triangle-cut

Here we verify a triangle cut of our one-loop four point integrand.

```

In[78]:= thisCut = {Atree[{k[1], k[2], l[1], l[2]}],
                    Atree[{-l[1], k[3], l[3]}],
                    Atree[{-l[3], k[4], -l[2]}]};

thisCutMassRules =
  {k[1]  $\rightarrow$  massive[k[1], m[1]], k[2]  $\rightarrow$  massive[k[2], m[1]], k[3]  $\rightarrow$  massive[k[3], m[2]],
   k[4]  $\rightarrow$  massive[k[4], m[2]], l[3]  $\rightarrow$  massive[l[3], m[2]]};

```

We'll need some conservation of momentum rules

```

In[80]:= masslessLegs =
  Select[Flatten[thisCut /. Atree[a__] => a /. -a_ => a] /. thisCutMassRules // Union,
    Head[#] != massive &];

In[81]:= thisCutPols =  $\epsilon$  /@masslessLegs;

In[82]:= theseCutRules =
  getIndepRules[thisCut /. thisCutMassRules, (thisCutMassRules /. Rule[b_, c_] =>
    (ulp[c, c] == (ulp[c, c] /. massive[i_, j_] => j /. ulp[0, 0] => 0)) // Flatten) ~
    Join~Map[ulp[#, #] == 0 &, masslessLegs]];
thesePolRules = getPolRules[thisCut /. thisCutMassRules, thisCutPols];

We introduce a function to just apply these rules as necessary:

In[84]:= backToBasis[expr_] := expr //. theseCutRules //. thesePolRules;

Conservation of momentum rules:

```

In[85]:= **theseCutRules**

```
Out[85]= {ulp[k[ms[4, m[2]]], l[ms[3, m[2]]]] → ulp[l[ms[3, m[2]]], l[ms[3, m[2]]]],
  ulp[k[ms[4, m[2]]], k[ms[4, m[2]]]] → ulp[l[ms[3, m[2]]], l[ms[3, m[2]]]],
  ulp[k[ms[3, m[2]]], l[ms[3, m[2]]]] → -ulp[l[ms[3, m[2]]], l[ms[3, m[2]]]],
  ulp[k[ms[3, m[2]]], k[ms[3, m[2]]]] → ulp[l[ms[3, m[2]]], l[ms[3, m[2]]]],
  ulp[k[ms[2, m[1]]], k[ms[3, m[2]]]] → -ulp[k[ms[2, m[1]]], k[ms[4, m[2]]]] -
    ulp[k[ms[3, m[2]]], k[ms[4, m[2]]]] - ulp[l[ms[3, m[2]]], l[ms[3, m[2]]]],
  ulp[k[ms[1, m[1]]], l[ms[3, m[2]]]] → -ulp[k[ms[2, m[1]]], l[ms[3, m[2]]]],
  ulp[k[ms[1, m[1]]], k[ms[4, m[2]]]] → -ulp[k[ms[2, m[1]]], k[ms[4, m[2]]]] -
    ulp[k[ms[3, m[2]]], k[ms[4, m[2]]]] - ulp[l[ms[3, m[2]]], l[ms[3, m[2]]]],
  ulp[k[ms[1, m[1]]], k[ms[3, m[2]]]] → ulp[k[ms[2, m[1]]], k[ms[4, m[2]]]],
  ulp[k[ms[1, m[1]]], k[ms[2, m[1]]]] → -ulp[k[ms[2, m[1]]], k[ms[2, m[1]]]] +
    ulp[k[ms[3, m[2]]], k[ms[4, m[2]]]] + ulp[l[ms[3, m[2]]], l[ms[3, m[2]]]],
  ulp[k[ms[1, m[1]]], k[ms[1, m[1]]]] → ulp[k[ms[2, m[1]]], k[ms[2, m[1]]]],
  ulp[m[2], m[2]] → ulp[l[ms[3, m[2]]], l[ms[3, m[2]]]],
  ulp[m[1], m[1]] → ulp[k[ms[2, m[1]]], k[ms[2, m[1]]]], ulp[l[2], l[ms[3, m[2]]]] → 0,
  ulp[k[ms[4, m[2]]], l[2]] → 0, ulp[k[ms[3, m[2]]], l[2]] →
    ulp[k[ms[3, m[2]]], k[ms[4, m[2]]]] + ulp[l[ms[3, m[2]]], l[ms[3, m[2]]]],
  ulp[k[ms[2, m[1]]], l[2]] → ulp[k[ms[2, m[1]]], k[ms[4, m[2]]]] -
    ulp[k[ms[2, m[1]]], l[ms[3, m[2]]]], ulp[k[ms[1, m[1]]], l[2]] →
    -ulp[k[ms[2, m[1]]], k[ms[4, m[2]]]] + ulp[k[ms[2, m[1]]], l[ms[3, m[2]]]] -
    ulp[k[ms[3, m[2]]], k[ms[4, m[2]]]] - ulp[l[ms[3, m[2]]], l[ms[3, m[2]]]],
  ulp[l[2], l[2]] → 0, ulp[l[1], l[ms[3, m[2]]]] → 0, ulp[k[ms[4, m[2]]], l[1]] →
    ulp[k[ms[3, m[2]]], k[ms[4, m[2]]]] + ulp[l[ms[3, m[2]]], l[ms[3, m[2]]]],
  ulp[k[ms[3, m[2]]], l[1]] → 0, ulp[k[ms[2, m[1]]], l[1]] →
    -ulp[k[ms[2, m[1]]], k[ms[4, m[2]]]] + ulp[k[ms[2, m[1]]], l[ms[3, m[2]]]] -
    ulp[k[ms[3, m[2]]], k[ms[4, m[2]]]] - ulp[l[ms[3, m[2]]], l[ms[3, m[2]]]],
  ulp[k[ms[1, m[1]]], l[1]] → ulp[k[ms[2, m[1]]], k[ms[4, m[2]]]] -
    ulp[k[ms[2, m[1]]], l[ms[3, m[2]]]],
  ulp[l[1], l[2]] → ulp[k[ms[3, m[2]]], k[ms[4, m[2]]]] +
    ulp[l[ms[3, m[2]]], l[ms[3, m[2]]]], ulp[l[1], l[1]] → 0}
```

Note that Mathematica chose a basis where  $ulp[l[ms[3, m[2]]], l[ms[3, m[2]]]]$  means  $m_2^2$  and  $ulp[k[ms[2, m[1]]], k[ms[2, m[1]]]]$  means  $m_1^2$ .

We can make this a little prettier.

```
In[86]:= Unprotect[ulp];
Format[ulp[l[ms[3, m[2]]], l[ms[3, m[2]]]] =
  DisplayForm[ RowBox[ {SuperscriptBox[SubscriptBox[m, 2], 2}]]]
Format[ulp[k[ms[2, m[1]]], k[ms[2, m[1]]]] =
  DisplayForm[ RowBox[ {SuperscriptBox[SubscriptBox[m, 1], 2}]]]
```

```
Out[87]//DisplayForm=
 $m_2^2$ 
```

```
Out[88]//DisplayForm=
 $m_1^2$ 
```

Polarization rules (recall graviton polarizations factorize into products of gluon polarizations):

```
In[89]:= thesePolRules
```

```
Out[89]:= {ulp[ε[-l[1]], ε[-l[1]]] → 0, ulp[ε[l[1]], ε[l[1]]] → 0,
  ulp[ε[-l[2]], ε[-l[2]]] → 0, ulp[ε[l[2]], ε[l[2]]] → 0,
  ulp[k[ms[3, m[2]]], ε[-l[1]]] → -ulp[l[ms[3, m[2]]], ε[-l[1]]],
  ulp[k[ms[1, m[1]]], ε[-l[1]]] → -ulp[k[ms[2, m[1]]], ε[-l[1]]] -
    ulp[k[ms[4, m[2]]], ε[-l[1]]] + ulp[l[ms[3, m[2]]], ε[-l[1]]],
  ulp[l[2], ε[-l[1]]] → ulp[k[ms[4, m[2]]], ε[-l[1]]] - ulp[l[ms[3, m[2]]], ε[-l[1]]],
  ulp[l[1], ε[-l[1]]] → 0,
  ulp[k[ms[3, m[2]]], ε[l[1]]] → -ulp[l[ms[3, m[2]]], ε[l[1]]],
  ulp[k[ms[1, m[1]]], ε[l[1]]] → -ulp[k[ms[2, m[1]]], ε[l[1]]] -
    ulp[k[ms[4, m[2]]], ε[l[1]]] + ulp[l[ms[3, m[2]]], ε[l[1]]],
  ulp[l[2], ε[l[1]]] → ulp[k[ms[4, m[2]]], ε[l[1]]] - ulp[l[ms[3, m[2]]], ε[l[1]]],
  ulp[l[1], ε[l[1]]] → 0,
  ulp[k[ms[4, m[2]]], ε[-l[2]]] → ulp[l[ms[3, m[2]]], ε[-l[2]]],
  ulp[k[ms[1, m[1]]], ε[-l[2]]] → -ulp[k[ms[2, m[1]]], ε[-l[2]]] -
    ulp[k[ms[3, m[2]]], ε[-l[2]]] - ulp[l[ms[3, m[2]]], ε[-l[2]]],
  ulp[l[2], ε[-l[2]]] → 0, ulp[l[1], ε[-l[2]]] →
    ulp[k[ms[3, m[2]]], ε[-l[2]]] + ulp[l[ms[3, m[2]]], ε[-l[2]]],
  ulp[k[ms[4, m[2]]], ε[l[2]]] → ulp[l[ms[3, m[2]]], ε[l[2]]],
  ulp[k[ms[1, m[1]]], ε[l[2]]] → -ulp[k[ms[2, m[1]]], ε[l[2]]] -
    ulp[k[ms[3, m[2]]], ε[l[2]]] - ulp[l[ms[3, m[2]]], ε[l[2]]], ulp[l[2], ε[l[2]]] →
    0, ulp[l[1], ε[l[2]]] → ulp[k[ms[3, m[2]]], ε[l[2]]] + ulp[l[ms[3, m[2]]], ε[l[2]]]}
```

Let's find the individual graphs contributing to each tree in the cut using the function `unOrderedGraphs`

```
In[90]:= theseGraphs = unOrderedGraphs[#{#}, thisCutMassRules] & /@ thisCut;
```

This will be a list of graphs for each tree, so a list of lists.

Recall our cut is: {Atree[{k[1], k[2], l[1], l[2]}], Atree[{-l[1], k[3], l[3]}], Atree[{-l[3], k[4], -l[2]}]}

We should expect 3 cubic graphs associated with the four point tree, and one cubic graph associated with each three point tree.

Here are the graphs contributing on every side of the cut.



Here are the graphs contributing to  $\text{Atree}[\{k[1], k[2], l[1], l[2]\}]$

In[91]:= **graphPlot /@ theseGraphs[[1]]**

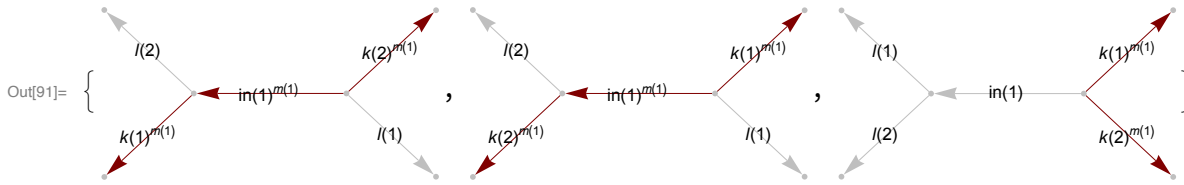

And the single graph contributing to:  $\text{Atree}[\{-l[1], k[3], l[3]\}]$

In[92]:= **graphPlot /@ theseGraphs[[2]]**

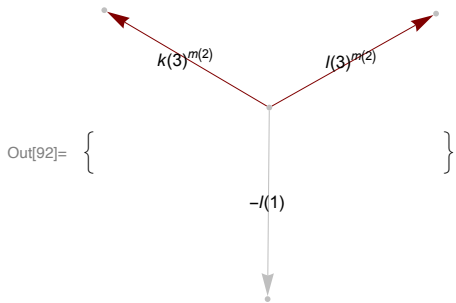

And the single graph contributing to:  $\text{Atree}[\{-l[3], k[4], -l[2]\}]$

In[93]:= **graphPlot /@ theseGraphs[[3]]**

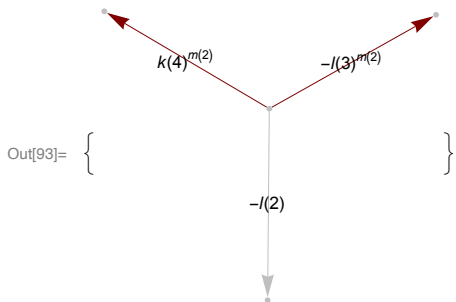

We'll dress these graphs with their tree amplitudes, then we'll have to perform the state sum over the gravitons.

In[94]:= **cutDressings =**

```
(Times @@ Table[Total[(getCutContribution[#1, treeGraph /@ allTreeGraphNames,
    gravityNumerator] &) /@ dat],
    {dat, theseGraphs}] /. theseCutRules /. thesePolRules) // Together;
```

In[95]:= **nums = ExpandAll[Numerator[cutDressings]];**

**denoms = Denominator[cutDressings];**

Sewing gravitons means summing over all valid graviton states:

In[97]:= **sewnCut = FixedPoint[(gravSewing[#, backToBasis] // Expand) &, nums] / denoms;**

Sewing ...

$$\varepsilon[l[1]]$$

$$\varepsilon[-l[1]]$$

Sewing ...

$$\varepsilon[l[2]]$$

$$\varepsilon[-l[2]]$$

The expression isn't entirely trivial

In[98]:= **Collect**[sewnCut /. dd → DD + 2, DD, FullSimplify] /. DD → dd - 2

$$\begin{aligned} \text{Out[98]= } & \left( \text{ulp}[k[\text{ms}[2, m[1]]], l[\text{ms}[3, m[2]]]]^2 \text{ulp}[k[\text{ms}[3, m[2]]], k[\text{ms}[4, m[2]]]] - \right. \\ & \text{ulp}[k[\text{ms}[2, m[1]]], k[\text{ms}[4, m[2]]]] m_2^2 (\text{ulp}[k[\text{ms}[2, m[1]]], k[\text{ms}[4, m[2]]]] + \\ & \text{ulp}[k[\text{ms}[3, m[2]]], k[\text{ms}[4, m[2]]]] + m_2^2) + \\ & \text{ulp}[k[\text{ms}[2, m[1]]], l[\text{ms}[3, m[2]]]] m_2^2 (2 \text{ulp}[k[\text{ms}[2, m[1]]], k[\text{ms}[4, m[2]]]] + \\ & \text{ulp}[k[\text{ms}[3, m[2]]], k[\text{ms}[4, m[2]]]] + m_2^2) \Big)^2 / \\ & (2 (\text{ulp}[k[\text{ms}[2, m[1]]], k[\text{ms}[4, m[2]]]] - \text{ulp}[k[\text{ms}[2, m[1]]], l[\text{ms}[3, m[2]]]]) \times \\ & (\text{ulp}[k[\text{ms}[3, m[2]]], k[\text{ms}[4, m[2]]]] + m_2^2) \times \\ & (\text{ulp}[k[\text{ms}[2, m[1]]], k[\text{ms}[4, m[2]]]] - \text{ulp}[k[\text{ms}[2, m[1]]], l[\text{ms}[3, m[2]]]] + \\ & \text{ulp}[k[\text{ms}[3, m[2]]], k[\text{ms}[4, m[2]]]] + m_2^2) \Big) - \\ & (m_2^2 (2 m_1^2 \text{ulp}[k[\text{ms}[2, m[1]]], l[\text{ms}[3, m[2]]]]^2 \\ & (\text{ulp}[k[\text{ms}[3, m[2]]], k[\text{ms}[4, m[2]]]] + m_2^2)^2 + \\ & (\text{ulp}[k[\text{ms}[2, m[1]]], k[\text{ms}[4, m[2]]]] - \text{ulp}[k[\text{ms}[2, m[1]]], l[\text{ms}[3, m[2]]]])^2 \\ & m_2^2 (\text{ulp}[k[\text{ms}[2, m[1]]], k[\text{ms}[4, m[2]]]] - \text{ulp}[k[\text{ms}[2, m[1]]], l[\text{ms}[3, m[2]]]] + \\ & \text{ulp}[k[\text{ms}[3, m[2]]], k[\text{ms}[4, m[2]]]] + m_2^2)^2) \Big) / (2 \times (-2 + dd) \\ & (\text{ulp}[k[\text{ms}[2, m[1]]], k[\text{ms}[4, m[2]]]] - \text{ulp}[k[\text{ms}[2, m[1]]], l[\text{ms}[3, m[2]]]]) \times \\ & (\text{ulp}[k[\text{ms}[3, m[2]]], k[\text{ms}[4, m[2]]]] + m_2^2) \times \\ & (\text{ulp}[k[\text{ms}[2, m[1]]], k[\text{ms}[4, m[2]]]] - \text{ulp}[k[\text{ms}[2, m[1]]], l[\text{ms}[3, m[2]]]] + \\ & \text{ulp}[k[\text{ms}[3, m[2]]], k[\text{ms}[4, m[2]]]] + m_2^2) \Big) + \frac{1}{2 (-2 + dd)^2} m_1^2 m_2^{22} \\ & \left( 2 + m_1^2 \left( \frac{1}{\text{ulp}[k[\text{ms}[2, m[1]]], k[\text{ms}[4, m[2]]]] - \text{ulp}[k[\text{ms}[2, m[1]]], l[\text{ms}[3, m[2]]]]} - \right. \right. \\ & \left. \left. 1 / (\text{ulp}[k[\text{ms}[2, m[1]]], k[\text{ms}[4, m[2]]]] - \text{ulp}[k[\text{ms}[2, m[1]]], l[\text{ms}[3, m[2]]]] + \right. \right. \\ & \left. \left. \text{ulp}[k[\text{ms}[3, m[2]]], k[\text{ms}[4, m[2]]]] + m_2^2) \right) \right) \Big) \end{aligned}$$

That expression must match what we get when we dress the contributing loop graphs with their relevant dressings and apply cut conditions to the resulting expression:

Here are the loop graphs contributing to this cut:

In[99]:= `graphPlot /@ unOrderedGraphs[thisCut, thisCutMassRules]`

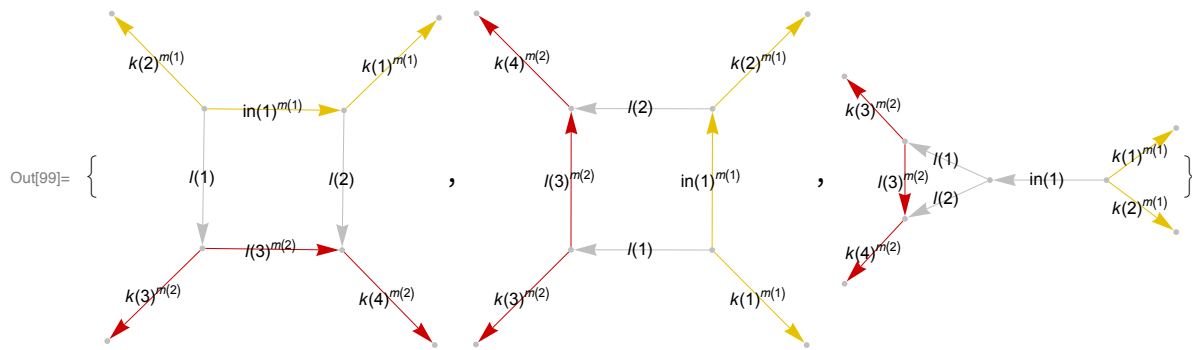

```

In[100]:= dressedCut =
  getCutContribution[#, oneLoopGraph /@ oneLoop4pGraphNames, gravityNumerator] & /@
    unOrderedGraphs[thisCut, thisCutMassRules] /.
      propagator[sq[a_]] -> ulp[a, a] // Total // backToBasis // Simplify
Out[100]= (2 × (-2 + dd) ulp[k[ms[2, m[1]]], l[ms[3, m[2]]]]3 m22
  (2 ulp[k[ms[2, m[1]]], k[ms[4, m[2]]]] + ulp[k[ms[3, m[2]]], k[ms[4, m[2]]]] + m22)
  ((-2 + dd) ulp[k[ms[3, m[2]]], k[ms[4, m[2]]]] + m22) +
  (-2 + dd) ulp[k[ms[2, m[1]]], l[ms[3, m[2]]]]4
  ((-2 + dd) ulp[k[ms[3, m[2]]], k[ms[4, m[2]]]]2 - m222) -
  2 ulp[k[ms[2, m[1]]], l[ms[3, m[2]]]] m222
  (2 ulp[k[ms[2, m[1]]], k[ms[4, m[2]]]] + ulp[k[ms[3, m[2]]], k[ms[4, m[2]]]] + m22) ×
  ((6 - 5 dd + dd2) ulp[k[ms[2, m[1]]], k[ms[4, m[2]]]]2 +
  m12 (ulp[k[ms[3, m[2]]], k[ms[4, m[2]]]] + m22) + (6 - 5 dd + dd2) ulp[
    k[ms[2, m[1]]], k[ms[4, m[2]]]] × (ulp[k[ms[3, m[2]]], k[ms[4, m[2]]]] + m22)) +
  m222 ((6 - 5 dd + dd2) ulp[k[ms[2, m[1]]], k[ms[4, m[2]]]]4 +
  2 × (6 - 5 dd + dd2) ulp[k[ms[2, m[1]]], k[ms[4, m[2]]]]3
  (ulp[k[ms[3, m[2]]], k[ms[4, m[2]]]] + m22) +
  m122 (ulp[k[ms[3, m[2]]], k[ms[4, m[2]]]] + m22)2 + 2 m12 ulp[k[ms[2, m[1]]],
    k[ms[4, m[2]]]] (ulp[k[ms[3, m[2]]], k[ms[4, m[2]]]] + m22)2 +
  ulp[k[ms[2, m[1]]], k[ms[4, m[2]]]]2 (ulp[k[ms[3, m[2]]], k[ms[4, m[2]]]] + m22)
  (2 m12 + (6 - 5 dd + dd2) (ulp[k[ms[3, m[2]]], k[ms[4, m[2]]]] + m22)) +
  ulp[k[ms[2, m[1]]], l[ms[3, m[2]]]]2 m22
  (-2 × (-2 + dd) ulp[k[ms[2, m[1]]], k[ms[4, m[2]]]]2
  ((-2 + dd) ulp[k[ms[3, m[2]]], k[ms[4, m[2]]]] + (7 - 2 dd) m22) - 2 × (-2 + dd) ulp[
    k[ms[2, m[1]]], k[ms[4, m[2]]]] × (ulp[k[ms[3, m[2]]], k[ms[4, m[2]]]] + m22)
  ((-2 + dd) ulp[k[ms[3, m[2]]], k[ms[4, m[2]]]] + (7 - 2 dd) m22) +
  (ulp[k[ms[3, m[2]]], k[ms[4, m[2]]]] + m22)
  ((6 - 5 dd + dd2) m22 (ulp[k[ms[3, m[2]]], k[ms[4, m[2]]]] + m22) -
    2 m12 ((-2 + dd) ulp[k[ms[3, m[2]]], k[ms[4, m[2]]]] + (-3 + dd) m22))) /
  (2 (-2 + dd)2 (ulp[k[ms[2, m[1]]], k[ms[4, m[2]]]] -
    ulp[k[ms[2, m[1]]], l[ms[3, m[2]]]] ×
    (ulp[k[ms[3, m[2]]], k[ms[4, m[2]]]] + m22) ×
    (ulp[k[ms[2, m[1]]], k[ms[4, m[2]]]] - ulp[k[ms[2, m[1]]], l[ms[3, m[2]]]] +
    ulp[k[ms[3, m[2]]], k[ms[4, m[2]]]] + m22))

```

This cut is satisfied if the difference between those expressions vanishes:

```

In[101]:= (sewnCut - dressedCut) // Together // Numerator

```

```

Out[101]= 0

```

# Using the one loop 5pt dressings

```
In[102]:= << "loop5pgravity.m";
```

```
In[103]:= graphPlot /@ (oneLoopGraph /@ oneLoop5pGraphNames /. internal -> i)
```

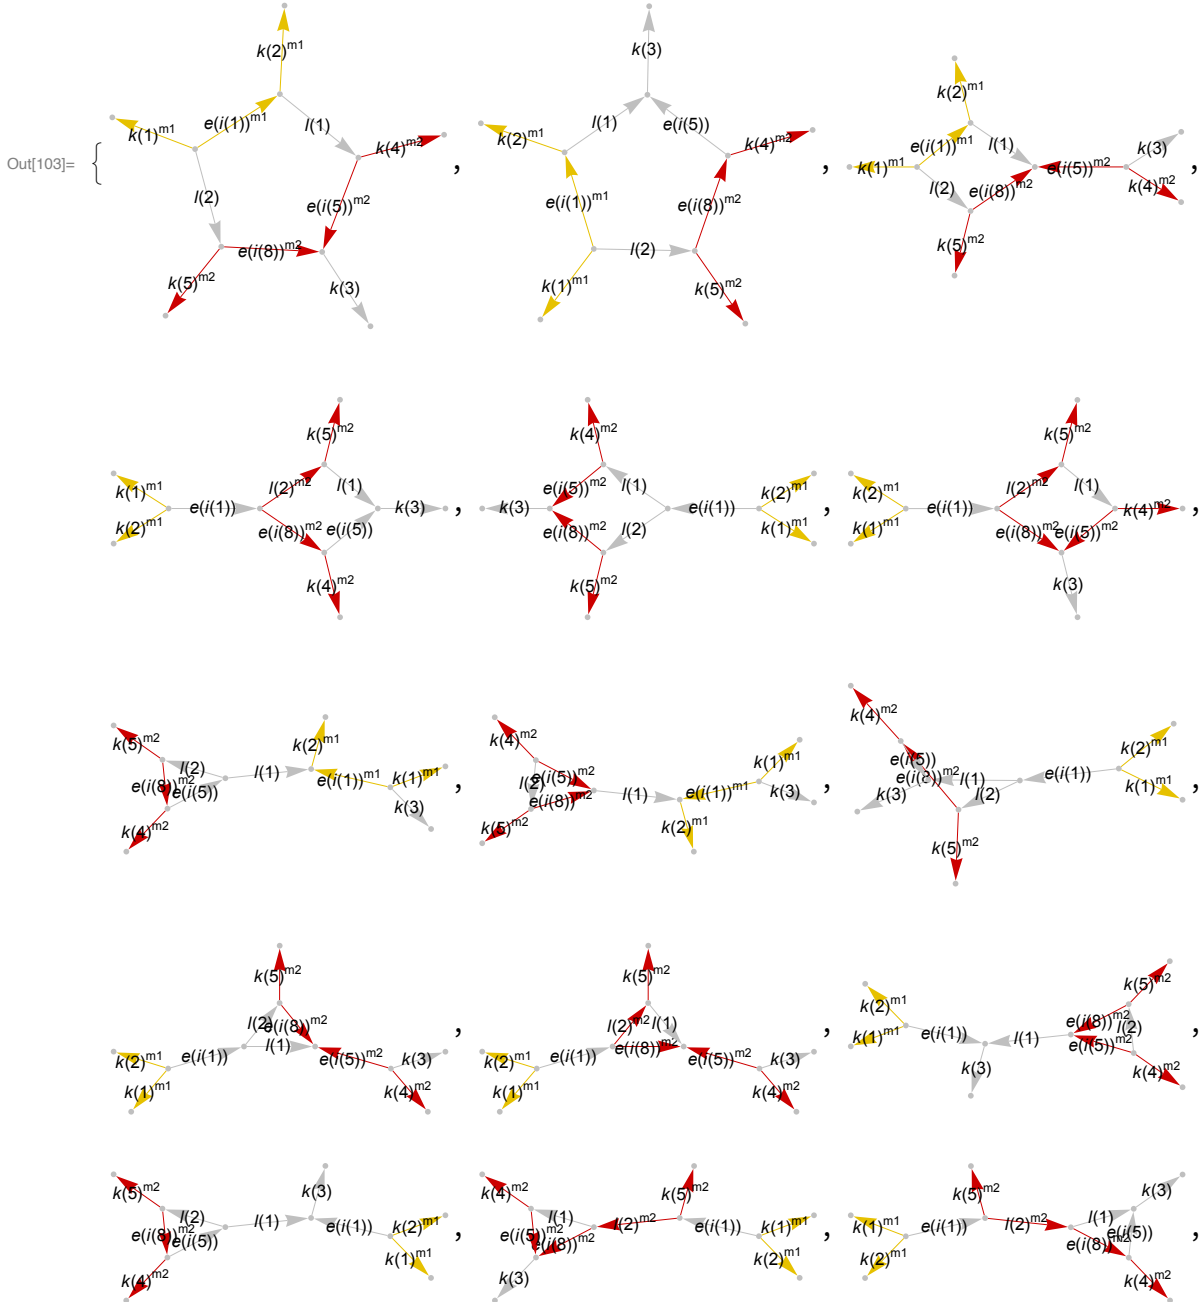

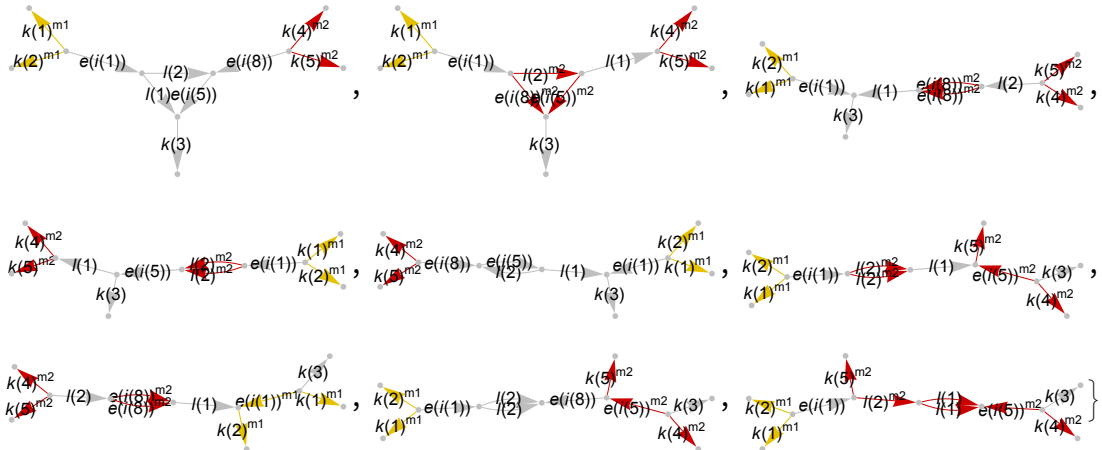

We can use these, for example, to verify a non-trivial box cut:

```
In[104]:= thisCut = {
  Atree[{k[1], k[2], l[1], l[2]}],
  Atree[{-l[1], k[3], l[3]}],
  Atree[{-l[3], k[4], l[4]}],
  Atree[{-l[4], k[5], -l[2]}]};
```

```
In[105]:= thisCutMassRules = {k[1] → massive[k[1], m[1]],
  k[2] → massive[k[2], m[1]],
  k[4] → massive[k[4], m[2]],
  k[5] → massive[k[5], m[2]],
  l[4] → massive[l[4], m[2]]};
```

We'll need some conservation of momentum rules

```
In[106]:= masslessLegs =
  Select[Flatten[thisCut /. Atree[a_] => a /. -a_ => a] /. thisCutMassRules // Union,
    Head[#] != massive &];
```

```
In[107]:= thisCutPols = ε /@ masslessLegs;
```

```
In[108]:= theseCutRules =
  getIndepRules[thisCut /. thisCutMassRules, (thisCutMassRules /. Rule[b_, c_] =>
    (ulp[c, c] == (ulp[c, c] /. massive[i_, j_] => j /. ulp[0, 0] => 0)) // Flatten) ~
    Join~Map[ulp[#, #] == 0 &, masslessLegs]];
thesePolRules = getPolRules[thisCut /. thisCutMassRules, thisCutPols];
backToBasis[expr_] := expr /. theseCutRules /. thesePolRules;
```

Conservation of momentum rules:

```
In[111]:= theseCutRules
```

```
Out[111]= {ulp[k[ms[5, m[2]]], l[ms[4, m[2]]]] → ulp[l[ms[4, m[2]]], l[ms[4, m[2]]]],
  ulp[k[ms[5, m[2]]], k[ms[5, m[2]]]] → ulp[l[ms[4, m[2]]], l[ms[4, m[2]]]],
```

```

ulp[k[ms[4, m[2]]], l[ms[4, m[2]]]] → -ulp[l[ms[4, m[2]]], l[ms[4, m[2]]]],
ulp[k[ms[4, m[2]]], k[ms[4, m[2]]]] → ulp[l[ms[4, m[2]]], l[ms[4, m[2]]]],
ulp[k[ms[1, m[1]]], k[ms[4, m[2]]]] → -ulp[k[ms[1, m[1]]], l[ms[4, m[2]]]] -
  ulp[k[ms[2, m[1]]], k[ms[4, m[2]]]] - ulp[k[ms[2, m[1]]], l[ms[4, m[2]]]] -
  ulp[k[ms[4, m[2]]], k[ms[5, m[2]]]] - ulp[l[ms[4, m[2]]], l[ms[4, m[2]]]],
ulp[k[ms[1, m[1]]], k[ms[2, m[1]]]] → -ulp[k[ms[1, m[1]]], k[ms[5, m[2]]]] +
  ulp[k[ms[1, m[1]]], l[ms[4, m[2]]]] - m12 - ulp[k[ms[2, m[1]]], k[ms[5, m[2]]]] +
  ulp[k[ms[2, m[1]]], l[ms[4, m[2]]]], ulp[k[ms[1, m[1]]], k[ms[1, m[1]]]] → m12,
ulp[m[2], m[2]] → ulp[l[ms[4, m[2]]], l[ms[4, m[2]]]], ulp[m[1], m[1]] → m12,
ulp[l[3], l[ms[4, m[2]]]] → 0, ulp[k[ms[5, m[2]]], l[3]] →
  ulp[k[ms[4, m[2]]], k[ms[5, m[2]]]] + ulp[l[ms[4, m[2]]], l[ms[4, m[2]]]],
ulp[k[ms[4, m[2]]], l[3]] → 0, ulp[k[ms[2, m[1]]], l[3]] →
  ulp[k[ms[2, m[1]]], k[ms[4, m[2]]]] + ulp[k[ms[2, m[1]]], l[ms[4, m[2]]]],
ulp[k[ms[1, m[1]]], l[3]] → -ulp[k[ms[2, m[1]]], k[ms[4, m[2]]]] -
  ulp[k[ms[2, m[1]]], l[ms[4, m[2]]]] - ulp[k[ms[4, m[2]]], k[ms[5, m[2]]]] -
  ulp[l[ms[4, m[2]]], l[ms[4, m[2]]]], ulp[l[3], l[3]] → 0,
ulp[l[2], l[ms[4, m[2]]]] → 0, ulp[k[ms[5, m[2]]], l[2]] → 0,
ulp[k[ms[4, m[2]]], l[2]] → ulp[k[ms[4, m[2]]], k[ms[5, m[2]]]] +
  ulp[l[ms[4, m[2]]], l[ms[4, m[2]]]], ulp[k[ms[2, m[1]]], l[2]] →
  ulp[k[ms[2, m[1]]], k[ms[5, m[2]]]] - ulp[k[ms[2, m[1]]], l[ms[4, m[2]]]],
ulp[k[ms[1, m[1]]], l[2]] → ulp[k[ms[1, m[1]]], k[ms[5, m[2]]]] -
  ulp[k[ms[1, m[1]]], l[ms[4, m[2]]]], ulp[l[2], l[3]] →
  ulp[k[ms[4, m[2]]], k[ms[5, m[2]]]] + ulp[l[ms[4, m[2]]], l[ms[4, m[2]]]],
ulp[l[2], l[2]] → 0, ulp[l[1], l[ms[4, m[2]]]] →
  -ulp[k[ms[1, m[1]]], l[ms[4, m[2]]]] - ulp[k[ms[2, m[1]]], l[ms[4, m[2]]]],
ulp[k[ms[5, m[2]]], l[1]] → -ulp[k[ms[1, m[1]]], k[ms[5, m[2]]]] -
  ulp[k[ms[2, m[1]]], k[ms[5, m[2]]]], ulp[k[ms[4, m[2]]], l[1]] →
  ulp[k[ms[1, m[1]]], l[ms[4, m[2]]]] + ulp[k[ms[2, m[1]]], l[ms[4, m[2]]]],
ulp[k[ms[2, m[1]]], l[1]] → ulp[k[ms[1, m[1]]], k[ms[5, m[2]]]] -
  ulp[k[ms[1, m[1]]], l[ms[4, m[2]]]], ulp[k[ms[1, m[1]]], l[1]] →
  ulp[k[ms[2, m[1]]], k[ms[5, m[2]]]] - ulp[k[ms[2, m[1]]], l[ms[4, m[2]]]],
ulp[l[1], l[3]] → 0, ulp[l[1], l[2]] →
  -ulp[k[ms[1, m[1]]], k[ms[5, m[2]]]] + ulp[k[ms[1, m[1]]], l[ms[4, m[2]]]] -
  ulp[k[ms[2, m[1]]], k[ms[5, m[2]]]] + ulp[k[ms[2, m[1]]], l[ms[4, m[2]]]],
ulp[l[1], l[1]] → 0, ulp[k[3], l[ms[4, m[2]]]] →
  -ulp[k[ms[1, m[1]]], l[ms[4, m[2]]]] - ulp[k[ms[2, m[1]]], l[ms[4, m[2]]]],
ulp[k[3], k[ms[5, m[2]]]] → -ulp[k[ms[1, m[1]]], k[ms[5, m[2]]]] -
  ulp[k[ms[2, m[1]]], k[ms[5, m[2]]]] - ulp[k[ms[4, m[2]]], k[ms[5, m[2]]]] -
  ulp[l[ms[4, m[2]]], l[ms[4, m[2]]]], ulp[k[3], k[ms[4, m[2]]]] →
  ulp[k[ms[1, m[1]]], l[ms[4, m[2]]]] + ulp[k[ms[2, m[1]]], l[ms[4, m[2]]]],
ulp[k[3], k[ms[2, m[1]]]] → ulp[k[ms[1, m[1]]], k[ms[5, m[2]]]] -
  ulp[k[ms[1, m[1]]], l[ms[4, m[2]]]] - ulp[k[ms[2, m[1]]], k[ms[4, m[2]]]] -
  ulp[k[ms[2, m[1]]], l[ms[4, m[2]]]], ulp[k[3], k[ms[1, m[1]]]] →
  ulp[k[ms[2, m[1]]], k[ms[4, m[2]]]] + ulp[k[ms[2, m[1]]], k[ms[5, m[2]]]] +

```

$$\begin{aligned}
& \text{ulp}[k[\text{ms}[4, m[2]]], k[\text{ms}[5, m[2]]]] + \text{ulp}[l[\text{ms}[4, m[2]]], l[\text{ms}[4, m[2]]]], \\
& \text{ulp}[k[3], l[3]] \rightarrow 0, \text{ulp}[k[3], l[2]] \rightarrow -\text{ulp}[k[\text{ms}[1, m[1]]], k[\text{ms}[5, m[2]]]] + \\
& \text{ulp}[k[\text{ms}[1, m[1]]], l[\text{ms}[4, m[2]]]] - \text{ulp}[k[\text{ms}[2, m[1]]], k[\text{ms}[5, m[2]]]] + \\
& \text{ulp}[k[\text{ms}[2, m[1]]], l[\text{ms}[4, m[2]]]] - \text{ulp}[k[\text{ms}[4, m[2]]], k[\text{ms}[5, m[2]]]] - \\
& \text{ulp}[l[\text{ms}[4, m[2]]], l[\text{ms}[4, m[2]]]], \text{ulp}[k[3], l[1]] \rightarrow 0, \text{ulp}[k[3], k[3]] \rightarrow 0\}
\end{aligned}$$

Polarization rules (recall graviton polarizations factorize into products of gluon polarizations):

In[112]:= **thesePolRules**

Out[112]= { $\text{ulp}[\varepsilon[-k[3]], \varepsilon[-k[3]] \rightarrow 0, \text{ulp}[\varepsilon[k[3]], \varepsilon[k[3]] \rightarrow 0,$   
 $\text{ulp}[\varepsilon[-l[1]], \varepsilon[-l[1]] \rightarrow 0, \text{ulp}[\varepsilon[l[1]], \varepsilon[l[1]] \rightarrow 0, \text{ulp}[\varepsilon[-l[2]], \varepsilon[-l[2]] \rightarrow 0,$   
 $\text{ulp}[\varepsilon[l[2]], \varepsilon[l[2]] \rightarrow 0, \text{ulp}[\varepsilon[-l[3]], \varepsilon[-l[3]] \rightarrow 0, \text{ulp}[\varepsilon[l[3]], \varepsilon[l[3]] \rightarrow 0,$   
 $\text{ulp}[k[\text{ms}[1, m[1]]], \varepsilon[-k[3]] \rightarrow -\text{ulp}[k[\text{ms}[2, m[1]]], \varepsilon[-k[3]] -$   
 $\text{ulp}[k[\text{ms}[4, m[2]]], \varepsilon[-k[3]] - \text{ulp}[k[\text{ms}[5, m[2]]], \varepsilon[-k[3]],$   
 $\text{ulp}[l[3], \varepsilon[-k[3]] \rightarrow \text{ulp}[k[\text{ms}[4, m[2]]], \varepsilon[-k[3]] + \text{ulp}[l[\text{ms}[4, m[2]]], \varepsilon[-k[3]],$   
 $\text{ulp}[l[2], \varepsilon[-k[3]] \rightarrow \text{ulp}[k[\text{ms}[5, m[2]]], \varepsilon[-k[3]] - \text{ulp}[l[\text{ms}[4, m[2]]], \varepsilon[-k[3]],$   
 $\text{ulp}[l[1], \varepsilon[-k[3]] \rightarrow \text{ulp}[k[\text{ms}[4, m[2]]], \varepsilon[-k[3]] + \text{ulp}[l[\text{ms}[4, m[2]]], \varepsilon[-k[3]],$   
 $\text{ulp}[k[3], \varepsilon[-k[3]] \rightarrow 0,$   
 $\text{ulp}[k[\text{ms}[1, m[1]]], \varepsilon[k[3]] \rightarrow -\text{ulp}[k[\text{ms}[2, m[1]]], \varepsilon[k[3]] -$   
 $\text{ulp}[k[\text{ms}[4, m[2]]], \varepsilon[k[3]] - \text{ulp}[k[\text{ms}[5, m[2]]], \varepsilon[k[3]],$   
 $\text{ulp}[l[3], \varepsilon[k[3]] \rightarrow \text{ulp}[k[\text{ms}[4, m[2]]], \varepsilon[k[3]] + \text{ulp}[l[\text{ms}[4, m[2]]], \varepsilon[k[3]],$   
 $\text{ulp}[l[2], \varepsilon[k[3]] \rightarrow \text{ulp}[k[\text{ms}[5, m[2]]], \varepsilon[k[3]] - \text{ulp}[l[\text{ms}[4, m[2]]], \varepsilon[k[3]],$   
 $\text{ulp}[l[1], \varepsilon[k[3]] \rightarrow \text{ulp}[k[\text{ms}[4, m[2]]], \varepsilon[k[3]] + \text{ulp}[l[\text{ms}[4, m[2]]], \varepsilon[k[3]],$   
 $\text{ulp}[k[3], \varepsilon[k[3]] \rightarrow 0,$   
 $\text{ulp}[k[\text{ms}[1, m[1]]], \varepsilon[-l[1]] \rightarrow -\text{ulp}[k[\text{ms}[2, m[1]]], \varepsilon[-l[1]] -$   
 $\text{ulp}[k[\text{ms}[5, m[2]]], \varepsilon[-l[1]] + \text{ulp}[l[\text{ms}[4, m[2]]], \varepsilon[-l[1]],$   
 $\text{ulp}[l[3], \varepsilon[-l[1]] \rightarrow \text{ulp}[k[\text{ms}[4, m[2]]], \varepsilon[-l[1]] + \text{ulp}[l[\text{ms}[4, m[2]]], \varepsilon[-l[1]],$   
 $\text{ulp}[l[2], \varepsilon[-l[1]] \rightarrow \text{ulp}[k[\text{ms}[5, m[2]]], \varepsilon[-l[1]] - \text{ulp}[l[\text{ms}[4, m[2]]], \varepsilon[-l[1]],$   
 $\text{ulp}[l[1], \varepsilon[-l[1]] \rightarrow 0, \text{ulp}[k[3], \varepsilon[-l[1]] \rightarrow$   
 $-\text{ulp}[k[\text{ms}[4, m[2]]], \varepsilon[-l[1]] - \text{ulp}[l[\text{ms}[4, m[2]]], \varepsilon[-l[1]],$   
 $\text{ulp}[k[\text{ms}[1, m[1]]], \varepsilon[l[1]] \rightarrow -\text{ulp}[k[\text{ms}[2, m[1]]], \varepsilon[l[1]] -$   
 $\text{ulp}[k[\text{ms}[5, m[2]]], \varepsilon[l[1]] + \text{ulp}[l[\text{ms}[4, m[2]]], \varepsilon[l[1]],$   
 $\text{ulp}[l[3], \varepsilon[l[1]] \rightarrow \text{ulp}[k[\text{ms}[4, m[2]]], \varepsilon[l[1]] + \text{ulp}[l[\text{ms}[4, m[2]]], \varepsilon[l[1]],$   
 $\text{ulp}[l[2], \varepsilon[l[1]] \rightarrow \text{ulp}[k[\text{ms}[5, m[2]]], \varepsilon[l[1]] - \text{ulp}[l[\text{ms}[4, m[2]]], \varepsilon[l[1]],$   
 $\text{ulp}[l[1], \varepsilon[l[1]] \rightarrow 0,$   
 $\text{ulp}[k[3], \varepsilon[l[1]] \rightarrow -\text{ulp}[k[\text{ms}[4, m[2]]], \varepsilon[l[1]] - \text{ulp}[l[\text{ms}[4, m[2]]], \varepsilon[l[1]],$   
 $\text{ulp}[k[\text{ms}[5, m[2]]], \varepsilon[-l[2]] \rightarrow \text{ulp}[l[\text{ms}[4, m[2]]], \varepsilon[-l[2]],$   
 $\text{ulp}[l[3], \varepsilon[-l[2]] \rightarrow \text{ulp}[k[\text{ms}[4, m[2]]], \varepsilon[-l[2]] + \text{ulp}[l[\text{ms}[4, m[2]]], \varepsilon[-l[2]],$   
 $\text{ulp}[l[2], \varepsilon[-l[2]] \rightarrow 0, \text{ulp}[l[1], \varepsilon[-l[2]] \rightarrow$   
 $-\text{ulp}[k[\text{ms}[1, m[1]]], \varepsilon[-l[2]] - \text{ulp}[k[\text{ms}[2, m[1]]], \varepsilon[-l[2]],$   
 $\text{ulp}[k[3], \varepsilon[-l[2]] \rightarrow -\text{ulp}[k[\text{ms}[1, m[1]]], \varepsilon[-l[2]] - \text{ulp}[k[\text{ms}[2, m[1]]],$   
 $\varepsilon[-l[2]] - \text{ulp}[k[\text{ms}[4, m[2]]], \varepsilon[-l[2]] - \text{ulp}[l[\text{ms}[4, m[2]]], \varepsilon[-l[2]],$   
 $\text{ulp}[k[\text{ms}[5, m[2]]], \varepsilon[l[2]] \rightarrow \text{ulp}[l[\text{ms}[4, m[2]]], \varepsilon[l[2]],$   
 $\text{ulp}[l[3], \varepsilon[l[2]] \rightarrow \text{ulp}[k[\text{ms}[4, m[2]]], \varepsilon[l[2]] + \text{ulp}[l[\text{ms}[4, m[2]]], \varepsilon[l[2]],$



```

ulp[l[2], ε[l[2]]] → 0,
ulp[l[1], ε[l[2]]] → -ulp[k[ms[1, m[1]]], ε[l[2]]] - ulp[k[ms[2, m[1]]], ε[l[2]]],
ulp[k[3], ε[l[2]]] → -ulp[k[ms[1, m[1]]], ε[l[2]]] - ulp[k[ms[2, m[1]]], ε[l[2]]] -
  ulp[k[ms[4, m[2]]], ε[l[2]]] - ulp[l[ms[4, m[2]]], ε[l[2]]],
ulp[k[ms[4, m[2]]], ε[-l[3]]] → -ulp[l[ms[4, m[2]]], ε[-l[3]]],
ulp[l[3], ε[-l[3]]] → 0,
ulp[l[2], ε[-l[3]]] → ulp[k[ms[5, m[2]]], ε[-l[3]]] - ulp[l[ms[4, m[2]]], ε[-l[3]]],
ulp[l[1], ε[-l[3]]] → -ulp[k[ms[1, m[1]]], ε[-l[3]]] - ulp[k[ms[2, m[1]]],
  ε[-l[3]]] - ulp[k[ms[5, m[2]]], ε[-l[3]]] + ulp[l[ms[4, m[2]]], ε[-l[3]]],
ulp[k[3], ε[-l[3]]] → -ulp[k[ms[1, m[1]]], ε[-l[3]]] - ulp[k[ms[2, m[1]]],
  ε[-l[3]]] - ulp[k[ms[5, m[2]]], ε[-l[3]]] + ulp[l[ms[4, m[2]]], ε[-l[3]]],
ulp[k[ms[4, m[2]]], ε[l[3]]] → -ulp[l[ms[4, m[2]]], ε[l[3]]], ulp[l[3], ε[l[3]]] → 0,
ulp[l[2], ε[l[3]]] → ulp[k[ms[5, m[2]]], ε[l[3]]] - ulp[l[ms[4, m[2]]], ε[l[3]]],
ulp[l[1], ε[l[3]]] → -ulp[k[ms[1, m[1]]], ε[l[3]]] - ulp[k[ms[2, m[1]]], ε[l[3]]] -
  ulp[k[ms[5, m[2]]], ε[l[3]]] + ulp[l[ms[4, m[2]]], ε[l[3]]],
ulp[k[3], ε[l[3]]] → -ulp[k[ms[1, m[1]]], ε[l[3]]] - ulp[k[ms[2, m[1]]], ε[l[3]]] -
  ulp[k[ms[5, m[2]]], ε[l[3]]] + ulp[l[ms[4, m[2]]], ε[l[3]]]

```

Here are the loop graphs contributing to this cut:

```
In[113]:= graphPlot /@ unOrderedGraphs[thisCut, thisCutMassRules]
```

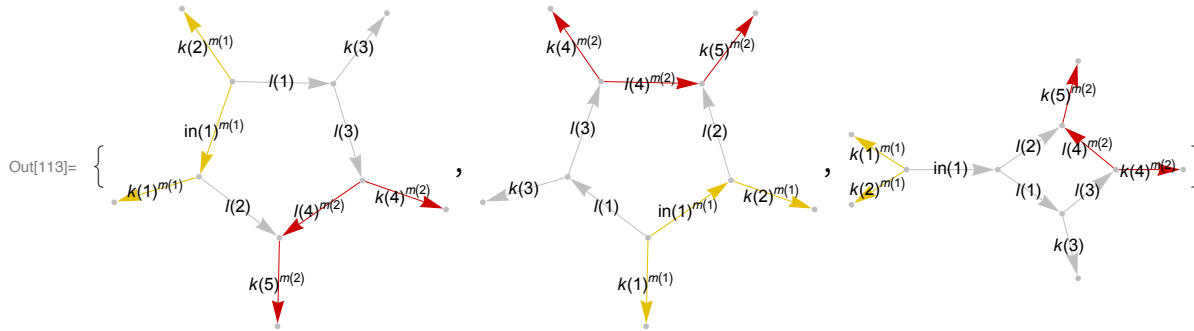

```
In[114]:= dressedCut =
  getCutContribution[#, oneLoopGraph /@ oneLoop5pGraphNames, gravityNumerator] & /@
    unorderedGraphs[thisCut, thisCutMassRules] //. propagator[sq[a_]] =>
      ulp[a, a] //. propagator[sq[a_] + b__] => ulp[a, a] + b // Total // backToBasis
```

Out[114]=

$$\left( \left( \left( \frac{\dots 1 \dots}{4} \right)^2 \left( \frac{\dots 1 \dots}{2} + \frac{\dots 1 \dots}{2} \right) + \frac{\dots 17 \dots}{2} + \frac{\dots 1 \dots}{2} \right)^2 - \frac{\frac{\dots 1 \dots}{4} \frac{\dots 1 \dots}{\dots 1 \dots^2} - \frac{\dots 1 \dots}{2} \frac{\left( \frac{\dots 1 \dots}{2} \right)}{(-2+dd)} \right) /$$

$$\left( 2 \left( -\text{ulp}[k[\text{ms}[1, m[1]]], k[\text{ms}[5, m[2]]]] + \text{ulp}[k[\text{ms}[1, m[1]]], l[\text{ms}[4, m[2]]]] - \text{ulp}[k[\text{ms}[2, \frac{\dots 1 \dots}{2}], \frac{\dots 1 \dots}{2}] + \text{ulp}[k[\text{ms}[2, m[1]]], l[\text{ms}[4, m[2]]]] \right) + \frac{\frac{\dots 1 \dots}{2}}{\frac{\dots 1 \dots}{2}} + \frac{\frac{\dots 1 \dots}{2}}{\frac{\dots 1 \dots}{2}} \right)$$

large output

[show less](#)[show more](#)[show all](#)[set size limit...](#)

```
In[115]:= dressedDots = dressedCut ~extractType~ ulp
```

```
Out[115]= {ulp[k[ms[1, m[1]]], k[ms[5, m[2]]]],
  ulp[k[ms[1, m[1]]], l[ms[4, m[2]]]], m1^2, ulp[k[ms[2, m[1]]], k[ms[4, m[2]]]],
  ulp[k[ms[2, m[1]]], k[ms[5, m[2]]]], ulp[k[ms[2, m[1]]], l[ms[4, m[2]]]],
  ulp[k[ms[2, m[1]]], ε[k[3]]], ulp[k[ms[4, m[2]]], k[ms[5, m[2]]]],
  ulp[k[ms[4, m[2]]], ε[k[3]]], ulp[k[ms[5, m[2]]], ε[k[3]]],
  ulp[l[ms[4, m[2]]], l[ms[4, m[2]]]], ulp[l[ms[4, m[2]]], ε[k[3]]]}
```

The expressions are large, so for expediency we'll compare on a set of momenta evaluated to random primes.

```
In[116]:= nDotRules = Map[#, RandomPrime[{10^3, 10^6}] &, dressedDots]
```

```
Out[116]= {ulp[k[ms[1, m[1]]], k[ms[5, m[2]]]] -> 636 553,
  ulp[k[ms[1, m[1]]], l[ms[4, m[2]]]] -> 798 443,
  m1^2 -> 25 367, ulp[k[ms[2, m[1]]], k[ms[4, m[2]]]] -> 419 261,
  ulp[k[ms[2, m[1]]], k[ms[5, m[2]]]] -> 193 493,
  ulp[k[ms[2, m[1]]], l[ms[4, m[2]]]] -> 786 661,
  ulp[k[ms[2, m[1]]], ε[k[3]]] -> 394 967, ulp[k[ms[4, m[2]]], k[ms[5, m[2]]]] -> 845 729,
  ulp[k[ms[4, m[2]]], ε[k[3]]] -> 741 593, ulp[k[ms[5, m[2]]], ε[k[3]]] -> 424 027,
  ulp[l[ms[4, m[2]]], l[ms[4, m[2]]]] -> 61 949, ulp[l[ms[4, m[2]]], ε[k[3]]] -> 648 019}
```

```

In[117]:= dressedCut /. nDotRules // Expand
Out[117]= - 
$$\frac{1\,784\,283\,138\,619\,023\,680\,574\,656\,373\,032\,944\,717\,366\,483\,801}{2\,265\,833\,909\,366\,130}$$


$$- \frac{110\,114\,073\,372\,627\,084\,548\,878\,919\,037\,432\,645\,889}{6\,001\,747\,970\,(-2 + dd)^2}$$


$$+ \frac{1\,108\,310\,711\,592\,292\,645\,077\,485\,151\,131\,707}{377\,529 \times (-2 + dd)}$$


$$+ \frac{5\,556\,489\,879\,935\,208\,872\,250\,895\,936\,414\,751\,966\,dd}{600\,174\,797\,(-2 + dd)^2}$$


```

Individual graphs contributing to each tree on the tree side:

```

In[118]:= theseGraphs = unOrderedGraphs[{}, thisCutMassRules] & /@ thisCut;

```

Here are the graphs contributing to every tree.

```

In[119]:= thisCut[[1]] /. thisCutMassRules

```

```

Out[119]= Atree[{massive[k[1], m[1]], massive[k[2], m[1]], l[1], l[2]}]

```

```

In[120]:= graphPlot /@ theseGraphs[[1]]

```

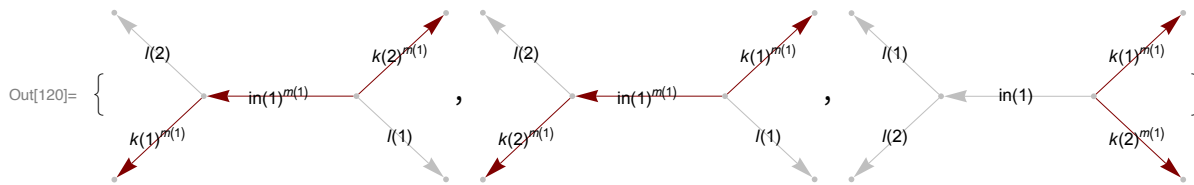

```

In[121]:= thisCut[[2]] /. thisCutMassRules

```

```

Out[121]= Atree[{-l[1], k[3], l[3]}]

```

```

In[122]:= graphPlot /@ theseGraphs[[2]]

```

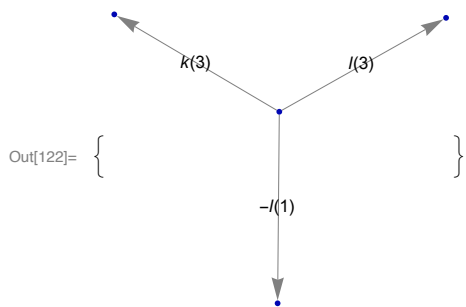

```

In[123]:= thisCut[[3]] /. thisCutMassRules

```

```

Out[123]= Atree[{-l[3], massive[k[4], m[2]], massive[l[4], m[2]]}]

```

```
In[124]:= graphPlot /@ theseGraphs[[3]]
```

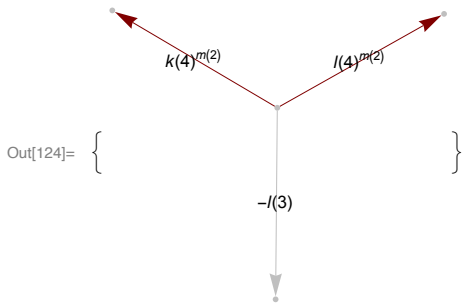

```
In[125]:= thisCut[[4]] /. thisCutMassRules
```

```
Out[125]= Atree[{-massive[l[4], m[2]], massive[k[5], m[2]], -l[2]}]
```

```
In[126]:= graphPlot /@ theseGraphs[[4]]
```

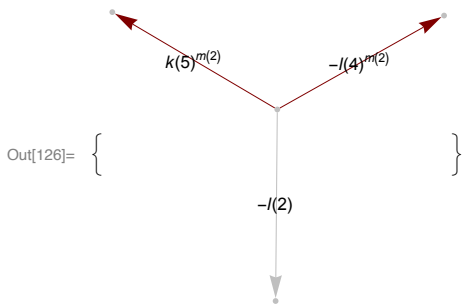

We'll dress these graphs with their amplitudes, then we'll have to perform the state sum over the gravitons.

```
In[127]:= cutDressings =
  (Times @@ Table[Total[(getCutContribution[#1, treeGraph /@ allTreeGraphNames,
    gravityNumerator] &) /@ dat],
    {dat, theseGraphs}] /. theseCutRules /. thesePolRules) // Together;
```

```
In[128]:= nums = ExpandAll[Numerator[cutDressings]];
```

```
denoms = Denominator[cutDressings];
```

Sewing gravitons means summing over all valid graviton states.

```
In[130]:= sewnCut = FixedPoint[gravSewing[#, backToBasis] &, nums] / denoms;
```

Sewing ...

$$\varepsilon[l[1]]$$

$$\varepsilon[-l[1]]$$

Sewing ...

$$\varepsilon[l[2]]$$

$$\varepsilon[-l[2]]$$

Sewing ...

$$\varepsilon[l[3]]$$

$$\varepsilon[-l[3]]$$

And evaluating numerically, we find sewing the trees is equivalent to our dressed graphs on this cut:

```
In[131]:= (sewnCut - dressedCut /. nDotRules // Together) === 0
```

```
Out[131]= True
```
